# Supplementary material for: An Efficient Approach to Achieve Compositionality using Optimized Multi-Version Object Based Transactional Systems
Source: arXiv:1905.01200 source file (2019-05-03)
Supplement: Supplementary file 2 [file appendix.tex]

\section*{Appendix}
\label{apn:appendix}

\appendix

\section{Detailed Pcode of MVOSTM}
\label{apn:rpcode}
%\vspace{-.3cm}

\subsection{Global DS}
\begin{lstlisting}{language = C++}
struct G_node{
int G_key;
struct G_vl;
G_lock;			
node G_knext;    
};
\end{lstlisting}

\begin{lstlisting}{language = C++}
struct G_vl{
int G_ts;
int G_val;
bool G_mark; 	
/*rvl stands for return value list*/
int G_rvl[];			
vl G_vnext;    
};
\end{lstlisting}

\subsection{Local DS}

\begin{lstlisting}{language = C++}
class L_txlog{
int L_t_id;			
STATUS L_tx_status;
vector <L_rec> L_list;
find();
getList();
};
\end{lstlisting}

\begin{lstlisting}{language = C++}
class L_rec{
int L_obj_id;
int L_key; 
int L_val;		
node* L_knext, G_pred, G_curr, node;
STATUS L_op_status;		
OP_NAME L_opn;
getOpn();	getPreds&Currs();  getOpStatus();
getKey&Objid();	getVal();	   getAptCurr();
setVal();	setPreds&Currs();  setOpStatus();   setOpn();
};
enum OP_NAME = {INSERT, DELETE, LOOKUP}
enum STATUS = {ABORT = 0, OK, FAIL, COMMIT}
\end{lstlisting}

\begin{table}[H]
	\centering
	\begin{tabular}{ || m{8em} | m{9cm}|| } 
		\hline
		\textbf{Functions} & \textbf{Description} \\ 
		\hline 		\hline
		setOpn() & set method name into transaction local log\\ 
		\hline
		setVal() & set value of the key into transaction local log\\ 
		\hline
		setOpStatus() & set status of method into transaction local log\\ 
		\hline
		setPred\&Curr() & set location of $G\_pred$ and $G\_curr$ according to the node corresponding to the key into transaction local log\\ 
		\hline
		getOpn() & get method name from transaction local log\\ 
		\hline
		getVal() & get value of the key from transaction local log\\ 
		\hline
		getOpStatus() & get status of the method from transaction local log\\ 
		\hline
		getKey\&Objid() & get key and obj\_id corresponding to the method from transaction local log\\ 
		\hline
		getPred\&Curr() & get location of $G\_preds$ and $G\_currs$ according to the node corresponding to the key from transaction local log \\ 
		\hline		
	\end{tabular}
	\caption{Description of accessing transaction local log methods}
	\label{tabel:1}
\end{table}

\begin{table}[H]
	\centering
	\begin{tabular}{ || m{2.3cm} | m{2.3cm} | m{2.3cm} | m{2.3cm} | m{2.3cm}|| } 
		\hline
		\textbf{p/q} & \textbf{\npins{}} & \textbf{\npdel{}} & \textbf{\npluk{}} & \textbf{\nptc} \\ 
		\hline 		
		\textbf{\npins{}} & + & + & + & +\\
		\hline
		\textbf{\npdel{}} & + & + & + & -\\
		\hline
		\textbf{\npluk{}} & + & + & + & -\\
		\hline
		\textbf{\nptc{}} & + & - & - & -\\
		\hline
	\end{tabular}
	\caption{Commutative table}
	\label{tabel:2}
\end{table}

%%%%%%%%%%%%%%%%%%%%%%%%%%%%%%%%%% STM_init()
 %Return the transaction id ($L\_t\_id$) at \Lineref{begin8}.

%Transaction id ($L\_t\_id$), object id (L\_obj\_id), node corresponding to the key (L\_key) and value(L\_val) are the inputs of this function.  

\cmnt{
\setlength{\textfloatsep}{0pt}

%%%%%%%%%%%%%%%%%%%%%%%%%%%%%%%%%%%%%%%%%%%%%%%%%%rv_method()%%%%%%%%%%%%%
\begin{algorithm} [H]
%\label{alg:llsearch} 
\scriptsize
\caption{\emph{\rvmt()} }
\setlength{\multicolsep}{0pt}
%\begin{multicols}{2}
\begin{algorithmic}[1]
\makeatletter\setcounter{ALG@line}{0}\makeatother
\Procedure{\rvmt{()}}{}
\If{(($m_{ij}(k)$ == \npluk{}) $||$ ($m_{ij}(k)$ == \npdel{}))}
\If{(k $\in$ local\_log(key))}
\State Update the local log \& return;
\Else
\State Search into the $CDS$ to identify the $preds$ \& $currs$ for key in \bn{} \& \rn.
\State Acquire the locks in increasing order.
\If{($!rv\_Validation()$)}
\State Release the locks and retry;
\ElsIf{(k $\notin$ $CDS$)} 
\State Create the new node in \rn{} and add the $T_0$ version in it. 
\EndIf
\State $find\_lts():$ Identify the version with largest TS as $T_j$ but less then TS($T_i$);
\State Add TS($T_i$) into $rvl$ of $T_j$;
\State Release the locks and update the local log;
\EndIf
\EndIf
\EndProcedure
\end{algorithmic}
%\end{multicols}
\end{algorithm}

%%%%%%%%%%%%%%%%%%%%%%%%%%%%%%%%%%%%%%%%%%%%%%%%%%rv_validation()%%%%%%%%%%%%%
\begin{algorithm} [H]
%\label{alg:llsearch} 
\scriptsize
\caption{\emph{rv\_Validation()} }
\setlength{\multicolsep}{0pt}
%\begin{multicols}{2}
\begin{algorithmic}[1]
\makeatletter\setcounter{ALG@line}{0}\makeatother
\Procedure{rv\_validation{()}}{}
\If{$((\bp.marked) || (\bc.marked) ||(\bp.\bn) \neq \bc || (\rp.\rn) \neq {\rc})$}
\State return $false$;
\Else 
\State return $true$;
\EndIf 
\EndProcedure
\end{algorithmic}
%\end{multicols}
\end{algorithm}

%%%%%%%%%%%%%%%%%%%%%%%%%%%%%%%%%%%%%%%%%%%%%%%%%%try_C()%%%%%%%%%%%%%
\begin{algorithm} [H]
%\label{alg:llsearch} 
\scriptsize
\caption{\emph{tryC()} }
\setlength{\multicolsep}{0pt}
%\begin{multicols}{2}
\begin{algorithmic}[1]
\makeatletter\setcounter{ALG@line}{0}\makeatother
\Procedure{tryC{()}}{}
\State Get the local log list for corresponding transaction;
\ForAll{(opn $\in$ local\_log\_list)}
\If{(($m_{ij}(k)$ == \npins{}) $||$ ($m_{ij}(k)$ == \npdel{}))}
\State Search into the $CDS$ to identify the $preds$ \& $currs$ for key in \bn{} \& \rn;
\State Acquire the locks in increasing order;
\If{($!rv\_Validation()$)}
\State Release the locks and retry;
\EndIf
\State $find\_lts():$ If (k $\in$ $CDS$) then identify the version with largest TS as $T_j$ but less then TS($T_i$);
\If{($!tryC\_Validation()$)}
\State return $Abort$;
\EndIf
\EndIf
\EndFor
\ForAll{(opn $\in$ local\_log\_list)}
\If{(($m_{ij}(k)$ == \npins{}) $||$ ($m_{ij}(k)$ == \npdel{}))}
\State $intraTransValidation():$ Update the preds and currs of consecutive operation working on same region.
\If{(k $\notin$ CDS)}
\State Create the new node in \rn{}, \bn{} and add the $T_0$ version in it;
\EndIf
\State $find\_lts():$ Identify the version with largest TS as $T_j$ but less then TS($T_i$);
\State Add TS($T_i$) into $rvl$ of $T_j$;
\State Update the local log;
\EndIf
\EndFor
%\EndFor
\State Release the locks;
\EndProcedure
\end{algorithmic}
%\end{multicols}
\end{algorithm}

%%%%%%%%%%%%%%%%%%%%%%%%%%%%%%%%%%%%%%%%%%%%%%%%%%tryC_validation()%%%%%%%%%%%%%
\begin{algorithm} [H]
%\label{alg:llsearch} 
\scriptsize
\caption{\emph{tryC\_Validation()} }
\setlength{\multicolsep}{0pt}
%\begin{multicols}{2}
\begin{algorithmic}[1]
\makeatletter\setcounter{ALG@line}{0}\makeatother
\Procedure{tryC\_validation{()}}{}
\ForAll {$T_k$ in $rvl$ of $T_j$}
\If{(TS($(T_k)$ $>$ TS($T_i$)))}
\State return $false$;
\EndIf 
\EndFor
\EndProcedure
\end{algorithmic}
%\end{multicols}
\end{algorithm}

%%%%%%%%%%%%%%%%%%%%%%%%%%%%%%%%%%%%%%%%%%%%%%%%%%Local Log Search()%%%%%%%%%%%%%
\begin{algorithm} [H]
\label{alg:llsearch} 
\scriptsize
\caption{\emph{MV-OSTM} Algorithm}
\setlength{\multicolsep}{0pt}
%\begin{multicols}{2}
\begin{algorithmic}[1]
\makeatletter\setcounter{ALG@line}{0}\makeatother
%\Procedure{STM local log search}{key} \label{lin:ll1}
\If{($G\_key$ $\in$ local\_log($L\_key$))} \label{lin:ll2}\Comment{Search into local log}
\If{$(($\textup{INSERT} $=$ \textup{$L\_opn$} $)||($ \textup{LOOKUP} $=$ \textup{$L\_opn$}$))$} \label{lin:ll3};
\State $L\_val$ $\gets$ $L\_getVal(L\_opn,L\_key)$ \label{lin:ll4};
\State $L\_op\_status$ $\gets$  $L\_getOpStatus$(L\_opn, L\_key) \label{lin:ll5};
%\State Update the local log.\label{lin:ll6}
			\ElsIf{$($\textup{DELETE} $=$ \textup{$L\_opn$}$)$} \label{lin:ll7}
			\State $L\_val$ $\gets$ NULL \label{lin:ll8}; 
			\State $L\_op\_status$ $\gets$ FAIL \label{lin:ll9}; 
\EndIf
\State Update the local log.
\State return $\langle L\_val$, $L\_op\_status \rangle$.\label{lin:ll10}
\EndIf

\State \Comment{Traversal phase}
\State $\bp$ $\gets$ $G\_head$ \label{lin:ltraversal2}; 
\State $\bc$ $\gets$ $\bp.\bn$ \label{lin:ltraversal3};
\While{$((\bc.key) < L\_key)$} \label{lin:ltraversal4};
\State $\bp$ $\gets$ $\bc$ \label{lin:ltraversal5};
\State $\bc$ $\gets$ $\bc.\bn$ \label{lin:ltraversal6};
\EndWhile \label{lin:ltraversal12}
\State $\rp$ $\gets$ $\bp$ \label{lin:ltraversal7}; 
\State $\rc$ $\gets$ $\rp.\rn$ \label{lin:ltraversal8};
\While{$((\rc.key) < L\_key)$} \label{lin:ltraversal9}
\State $\rp$ $\gets$ $\rc$ \label{lin:ltraversal10};
\State $\rc$ $\gets$ $\rc.\rn$ \label{lin:ltraversal11};
\EndWhile \label{lin:ltraversal14}
\State Update the \preds{} and \currs{} into local log.
\State \Comment{Validation phase}
\If{(($\bp$.marked) || ($\bc$.marked) ||($\bp.\bn$) $\neq$ $\bc$ || ($\rp.\rn$) $\neq$ {$\rc$})}\Comment{Validation}
\State return $\langle RETRY \rangle$;
\Else
\State return $\langle OK \rangle$;
\EndIf
\State /*Find the largest time-stamp but less then itself($T_i$).*/
\State $find\_lts$(max(closest\_tuple(TS($T_j$))) $<$ TS($T_i$))
\ForAll {($T_k$ $\in$ rvl($T_i$))}
\If{(TS($T_i$) < TS($T_k$))}
\State return $\langle ABORT \rangle$;
\Else
\State return $\langle OK \rangle$;
\end{algorithmic}
%\end{multicols}
\end{algorithm}

%%%%%%%%%%%%%%%%%%%%%%%%%%%%%%%%%%%%%%%%%%%%%%%%%%%%%%%%%%%%%%%%%%%%%%%%%%%%%%%%%%%%%%%%%%%%%%%%%%%%%%
%%%%%%%%%%%%%%%%%%%%%%%%%%%%%%%%%%%%%%%%%%%%%%%%%%%%%%%%%%%%%%%%%%%%%%%%%%
%-----------------------------------------TryCommit----------------------------------%---------
%----
%%%%%%%%%%%%%%%%%%%%%%%%%%%%%%%%%%%%%%%%%%%%%%%%%%%%%%%%%%%%%%%%%%%%%%%%%%

\begin{algorithm}[H]
\scriptsize
	\caption{\tabspace[0.2cm] STM $tryC()$ }
	\label{algo:trycommit}
	\setlength{\multicolsep}{0pt}
		%\begin{multicols}{2}
	\begin{algorithmic}[1]
\makeatletter\setcounter{ALG@line}{33}\makeatother
		\Procedure{STM tryC}{($L\_t\_id$)} \label{lin:tryc1}
    \State $L\_list$ $\gets$ $getList$($L\_t\_id$) \label{lin:tryc3};
		\While{$(\textbf{$L\_rec_{i} \gets \textup{next}(L\_list$}))$} \label{lin:tryc5}
		\State ($L\_key, L\_obj\_id$) $\gets$ \llgkeyobj{} \label{lin:tryc6};
		\State \lsls{$COMMIT \downarrow$} \label{lin:tryc8};
			
		\If {$((\bc.key = L\_key) \& (\checkv(L\_t\_id \downarrow,\bc \downarrow) = FALSE))$}\label{lin:tryc9}
\State Unlock all the variables;\label{lin:tryc10}
\State return $ABORT$;\label{lin:tryc11}
\ElsIf {$((\rc.key = L\_key) \& (\checkv(L\_t\_id \downarrow,\rc \downarrow) = FALSE))$}\label{lin:stryc9}
\State Unlock all the variables;\label{lin:stryc10}
\State return $ABORT$;\label{lin:stryc11}

\EndIf;\label{lin:tryc12}
		\State \llspc{} \label{lin:tryc14};
		\EndWhile \label{lin:tryc15}
	\While{$(\textbf{$L\_rec_{i} \gets \textup{next}(L\_list$}))$} \label{lin:tryc17}
		\State ($L\_key, L\_obj\_id$) $\gets$ \llgkeyobj{} \label{lin:tryc18};
		\State $L\_opn$ $\gets$ $(L\_rec)_{i}$.$L\_opn$ \label{lin:tryc20};
		\State intraTransValdation($L\_rec_{i} \downarrow$, $\preds \uparrow$, $\currs \uparrow$) \label{lin:tryc42};
		\If{$($\textup{INSERT} $=$ \textup{$L\_opn$}$)$} \label{lin:tryc22}
		\If{$(\bc.key) = L\_key)$} \label{lin:tryc23}
	\State insert $v\_tuple \langle L\_t\_id,val,F,NULL,NULL \rangle$ into $G\_curr.vl$ in the increasing order;	\label{lin:tryc24}
	
	\ElsIf{$(\rc.key) = L\_key)$} \label{lin:stryc23}
	\State \lslins{$RL\_BL \downarrow$} \label{lin:stryc24}
	\State insert $v\_tuple \langle L\_t\_id,val,F,NULL,NULL \rangle$ into $G\_curr.vl$ in the increasing order;	\label{lin:stryc25}
	
		\Else \label{lin:tryc25}
		\State \lslins{$BL \downarrow$} \label{lin:tryc27};
		\State insert $v\_tuple \langle L\_t\_id,val,F,NULL,NULL \rangle$ into $node.vl$ in the increasing order;	\label{lin:tryc28}
	\EndIf \label{lin:tryc29}
\ElsIf{$($\textup{DELETE} $=$ $L\_opn)$} \label{lin:tryc31}
	\If{$(\bc.key) = L\_key)$} \label{lin:tryc33}
		\State insert $v\_tuple \langle L\_t\_id,NULL,T,NULL,NULL \rangle$ into $G\_curr.vl$ in the increasing order;	\label{lin:tryc34}
			\State \lsldel{} \label{lin:stryc35};
		\EndIf \label{lin:tryc39}
	
		\EndIf \label{lin:tryc40}
		\EndWhile \label{lin:tryc43}
        \State \rlsol{} \label{lin:tryc45};  
        \State $L\_tx\_status$ $\gets$ OK \label{lin:tryc47};
		\State return $\langle L\_tx\_status\rangle$\label{lin:tryc48};
		\EndProcedure \label{lin:tryc49}
	\end{algorithmic}
	%	\end{multicols}
\end{algorithm}

}

%%%%%%%%%%%%%%%%%%%%%%%%%%%%%%%%%% STM_init()

\begin{algorithm} 
\label{alg:init} 
\scriptsize

\caption{STM $\init()$: This method invokes at the start of the STM system. Initialize the global counter ($\cnt$) as 1 at \Lineref{init1} and return it.}
\setlength{\multicolsep}{0pt}
%\begin{multicols}{2}
\begin{algorithmic}[1]
\makeatletter\setcounter{ALG@line}{52}\makeatother	
\Procedure{STM init}{$\cnt \uparrow$}
\cmnts{Initializing the global counter}
\State $\cnt$ $\gets$ 1; \label{lin:init1}
\cmnt{
\ForAll {key $G\_k$ used by the STM System}
%\State /* $T_0$ is initializing key $k$ */
\State /*$T_0$ is initializing key $k$*/
\State add $\langle 0, 0, T, NULL, NULL \rangle$ to $G\_k.vl$;  \label{lin:init} %\Comment{Implies that $T_0$ has initialized $x$}
\EndFor;
}
\State return $\langle \cnt \rangle$; 
\EndProcedure
\end{algorithmic}
	
%	\end{multicols}
\end{algorithm}

\cmnt{
%%%%%%%%%%%%%%%%%%%%%%%%%%%%%%%%%%%%%%%%%%%%%Traversal Phase%%%%%%%%%%%%%%%%%%%%%%%
\begin{algorithm}[H]
\scriptsize
	\caption{list\_traversal() : It finds the location of the node corresponding to the key in underlying DS. First it identifies the node in \bn{} then in \rn{}. After finding the appropriate $\preds$ and $\currs$ corresponding to the key, it acquires the locks and validate it.}
	\label{algo:traversal}
	\setlength{\multicolsep}{0pt}
		%\begin{multicols}{2}
	\begin{algorithmic}[1]
	\makeatletter\setcounter{ALG@line}{166}\makeatother	
	\Procedure{list\_traversal}{$L\_Bucket\_id, L\_key$} \label{lin:ltraversal1}

%\cmnts{By default setting the $L\_op\_status$ as RETRY}\label{lin:lslsearch2}
	    %\State STATUS $L\_op\_status$ $\gets$ RETRY; \label{lin:lslsearch3}
	 %\cmnts{Identify the \preds and \currs for node corresponding to the key if $L\_op\_status$ is RETRY}\label{lin:lslsearch4}   
		%\While{($L\_op\_status$ = \textup{RETRY})} \label{lin:lslsearch5}
	%	\cmnts{Get the head of the bucket in chaining hash-table with the help of $L\_obj\_id$ and $L\_key$}\label{lin:lslsearch6}
		%\State $G\_head$ $\gets$ \glslhead \label{lin:lslsearch7};
	%	\cmnts{Initialize $\bp$ to head}\label{lin:lslsearch8}
		\State $\bp$ $\gets$ $G\_head$ \label{lin:ltraversal2}; 
	%	\cmnts{Initialize $\bc$ to $\bp.\bn$}\label{lin:lslsearch10}
		\State $\bc$ $\gets$ $\bp.\bn$ \label{lin:ltraversal3};
	%	\cmnts{Searching node corresponding to the key into \bn}
		\While{$((\bc.key) < L\_key)$} \label{lin:ltraversal4};
		\State $\bp$ $\gets$ $\bc$ \label{lin:ltraversal5};
				
		\State $\bc$ $\gets$ $\bc.\bn$ \label{lin:ltraversal6};
			
	%\EndWhile \label{lin:lslsearch15}
		
%		\cmnts{Initialize $\rp$ to head}\label{lin:slslsearch8}
		\State $\rp$ $\gets$ $\bp$ \label{lin:ltraversal7}; 
%		\cmnts{Initialize $\rc$ to $\rp.\rn$}\label{lin:slslsearch10}
		\State $\rc$ $\gets$ $\rp.\rn$ \label{lin:ltraversal8};
	%	\cmnts{Searching node corresponding to the key into \rn}
		\While{$((\rc.key) < L\_key)$} \label{lin:ltraversal9}
		\State $\rp$ $\gets$ $\rc$ \label{lin:ltraversal10};
				
		\State $\rc$ $\gets$ $\rc.\rn$ \label{lin:ltraversal11};
			
		\EndWhile \label{lin:ltraversal12}

		%\State    /*get the value*/
		%\State $L\_val$ $\gets$ $G\_curr.value$
		%\cmnts{Acquire the locks on increasing order of keys}\label{lin:lslsearch16}
	    \State acquirePred\&CurrLocks($ \preds$, $ \currs$); \label{lin:ltraversal13}
%\cmnts{Method validation to identify the changes done by concurrent conflicting method}\label{lin:lslsearch19}
		%\State methodValidation($\preds$ $\downarrow$, $\currs$ $\downarrow$, $L\_op\_status \uparrow$)\label{lin:lslsearch20};	
		%\State $op\_status$ $\gets$ \validation \label{lin:lslsearch21};
%\cmnts{If $L\_op\_status$ is RETRY then release all the locks}		\label{lin:lslsearch21}
	%	\If{(($L\_op\_status$ = \textup{RETRY}))} \label{lin:lslsearch22}
	   % \State releasePred\&CurrLocks($ \preds \downarrow$, $ \currs \downarrow$);
	    %\EndIf \label{lin:lslsearch25}
			
		\EndWhile \label{lin:ltraversal14}
		
		\State return $\langle G\_preds[], G\_currs[]\rangle$ \label{lin:ltraversal15};
	
	\EndProcedure \label{lin:ltraversal16}
	
	\end{algorithmic}
	%	\end{multicols}
\end{algorithm}
%\end{spacing}
}

%%%%%%%%%%%%%%%%%%%%%%%%%%%%%%%%%% STM_begin()
\begin{algorithm} 
\label{alg:begin} 
\scriptsize
\caption{STM $begin()$: It invoked by a thread to being a new transaction $T_i$. It creates transaction local log and allocate unique id at \Lineref{begin3} and \Lineref{begin5} respectively.}
\setlength{\multicolsep}{0pt}
%\begin{multicols}{2}
\begin{algorithmic}[1]
\makeatletter\setcounter{ALG@line}{88}\makeatother
\Procedure{STM begin}{$\cnt \downarrow$, $L\_t\_id \uparrow$} \label{lin:begin1}
\cmnts{Creating a local log for each transaction}\label{lin:begin2}
\State \txll $\gets$ create new \txllf;  \label{lin:begin3}
%\State /*Acquiring lock on live set of transaction*/
%\State $\livetx.lock()$;  
\cmnts{Getting transaction id ($L\_t\_id$) from $\cnt$}\label{lin:begin4}
\State \txll.$L\_t\_id$ $\gets$ $\cnt$;  \label{lin:begin5}
\cmnts{Incremented global counter atomically $\cnt$}\label{lin:begin6}
\State $\cnt$ $\gets$ \gi; //$\Phi_{lp}(Linearization Point)$ \label{lin:begin7}
%\State add $t\_id$ to $\livetx$; 
%\State /*Release lock on live set of transaction*/
%\State $\livetx.unlock()$; 
\State return $\langle L\_t\_id \rangle$; \label{lin:begin8}
\EndProcedure\label{lin:begin9}
\end{algorithmic}
%\end{multicols}
\end{algorithm}

%%%%%%%%%%%%%%%%%%%%%%%%%%%%%%%% STM_ Insert()

\begin{algorithm}[H]

	\caption{STM $insert():$ Optimistically, the actual insertion will happen in the \nptc{} method. First, it will identify the node corresponding to the key in local log. If the node exists then it just update the local log with useful information like value, operation name and status for the node corresponding to the key at \Lineref{insert8}, \Lineref{insert9} and \Lineref{insert10} respectively for later use in \nptc{}. Otherwise, it will create a local log and update it.}
    \scriptsize
\setlength{\multicolsep}{0pt}
%\begin{multicols}{2}
	\label{algo:insert}
	\begin{algorithmic}[1]
	\makeatletter\setcounter{ALG@line}{97}\makeatother
	\Procedure{STM insert}{$L\_t\_id \downarrow, L\_obj\_id \downarrow, L\_key \downarrow, L\_val \downarrow$}\label{lin:insert1}
	\cmnts{First identify the node corresponding to the key into local log using $find()$ funciton}\label{lin:insert2}
		\If{$(!$\txlfind$)$}\label{lin:insert3}
		\cmnts{Create local log record and append it into increasing order of keys} \label{lin:insert4}
		\State $L\_rec$ $\gets$ create new $L\_rec \langle L\_obj\_id, L\_key \rangle$; \label{lin:insert5}
		\EndIf \label{lin:insert6}
		\cmnts{Updating the local log} \label{lin:insert7}		\State \llsval{$L\_val \downarrow$};//$\Phi_{lp} (Linearization Point)$ \label{lin:insert8}
		\State \llsopn{$INSERT \downarrow$}; \label{lin:insert9}
		\State \llsopst{$OK \downarrow$}; \label{lin:insert10}
		\State return $\langle void \rangle$; \label{lin:insert11} 
    	%\State loclog.setOpStatus$(obj\_id \downarrow, key \downarrow, OK \downarrow)$;
    \EndProcedure	\label{lin:insert12}
	\end{algorithmic}
%\end{multicols}	
\end{algorithm}

%%%%%%%%%%%%%%%%%%%%%%%%%%%%%%%%%%%%%%%%%%%%%%%%%%%%%%%%%%%%%%%%%%%%%%%%%%
%-----------------------------------------STM\_LOOKUP-------------------------------------%------
%----
%%%%%%%%%%%%%%%%%%%%%%%%%%%%%%%%%%%%%%%%%%%%%%%%%%%%%%%%%%%%%%%%%%%%%%%%%%
%\begin{spacing}{2}
\begin{algorithm}[H]
	%\algsetup{linenosize=\tiny}
	
	\caption{\tabspace[0.2cm] STM $lookup_{i}()$: If \npluk{} is not the first method on a particular key means if its a subsequent method of the same transaction on that key then first it will search into the local log from \Lineref{lookup3} to \Lineref{lookup14}. If the previous method on the same key of same transaction was insert or lookup (from \Lineref{lookup7} to \Lineref{lookup9}) then \npluk{} will return the value and operation status based on previous operation value and status. If the previous method on the same key of same transaction was delete (from \Lineref{lookup11} to \Lineref{lookup13}) then \npluk{} will return the value and operation status as NULL and FAIL respectively. If \npluk{} is the first method on that key (from \Lineref{lookup16} to \Lineref{lookup22}) then it will identify the location of node corresponding to the key in underlying DS with the help of \nplsls{} inside the \npcld{} method at \Lineref{lookup17}.} %: If the transaction to which this operation belongs has locally done an operation on the same key then returns apt value and status(wrt the previous local operation). Else do the \nplsls{} to find the correct location of the key and validate it.
		%\emph{DESCP}\tabspace: If the Tx has locally done an operation returns apt value and status else does TO \tabspace[2.2cm] and method validation traversal phase in only.\\
		%\emph{IN}\tabspace \tabspace[0.72cm]: $obj\_id$, $key$\\
		%\emph{OUT}\tabspace \tabspace[0.37cm]: $value$, $op\_status$     }
	\scriptsize
	\setlength{\multicolsep}{0pt}
%	\begin{multicols}{2}
		
		\label{algo:lookup}
		%	\setlength{\multicolsep}{0pt}
		%	\begin{multicols}{2}
		
		\begin{algorithmic}[1]
			\makeatletter\setcounter{ALG@line}{109}\makeatother
			\Procedure{STM lookup}{$L\_t\_id \downarrow, L\_obj\_id \downarrow, L\_key \downarrow, L\_val \uparrow, L\_op\_status \uparrow$} \label{lin:lookup1}
			%\State $op\_status$ $\gets$ RETRY \label{lin:lookup2};
			\cmnts{First identify the node corresponding to the key into local log}\label{lin:lookup2}
			\If{$($\txlfind$)$} \label{lin:lookup3}
			\cmnts{Getting the previous operation's name}\label{lin:lookup4}
			\State $L\_opn$ $\gets$ \llgopn{} \label{lin:lookup5}; %\Comment{$\Phi_{lp}$}
			\cmnts{If previous operation is insert/lookup then get the value/op\_status based on the previous operations value/op\_status}\label{lin:lookup6}
			\If{$(($\textup{INSERT} $=$ \textup{$L\_opn$} $)||($ \textup{LOOKUP} $=$ \textup{$L\_opn$}$))$} \label{lin:lookup7}
			
			\State $L\_val$ $\gets$ \llgval{} \label{lin:lookup8};
			\State $L\_op\_status$ $\gets$  $L\_rec.L\_getOpStatus$($L\_obj\_id \downarrow, L\_key \downarrow$) \label{lin:lookup9};
			\cmnts{If previous operation is delete then set the value as NULL and op\_status as FAIL}\label{lin:lookup10}
			\ElsIf{$($\textup{DELETE} $=$ \textup{$L\_opn$}$)$} \label{lin:lookup11}
			\State $L\_val$ $\gets$ NULL \label{lin:lookup12}; 
			\State $L\_op\_status$ $\gets$ FAIL \label{lin:lookup13}; 
			\EndIf \label{lin:lookup14}
			%	\EndIf \label{lin:lookup11}
			\Else \label{lin:lookup15}
			\cmnts{ Common function for \rvmt{}, if node corresponding to the key is not part of local log}\label{lin:lookup16}
			\State \cld{};\label{lin:lookup17}
			\cmnt{		
				%\State $op\_status $ $\gets$ lslSearch($obj\_id$ $\downarrow$, $key$ $\downarrow$, $preds[]$ $\uparrow$, $currs[]$ $\uparrow$, $value_{BL}$ $\uparrow$, $RV$ $\downarrow$);	
				\State    /*if key is not present in local log then search in underlying DS with the help of list\_lookup*/
				\State \lsls{} \label{lin:lookup13}; 
				%State    /*if list\_lookup return op\_status as ABORT then method will return ABORT*/
				%If{$(op\_status_{ll}$ $=$ \textup{ABORT}$)$} \label{lin:lookup14}
				%			\State release all the locks
				%State \handlea{} \label{lin:lookup15}; 
				%Else \label{lin:lookup16}
				%			\State    /*check node corresponding to the key is part of underlying DS or not*/	
				%			\If{$((G\_curr.key) == L\_key)$} \label{lin:lookup17}
				\State /*From $G\_k.vls$, identify the right $version\_tuple$*/ 
				\State \find($L\_t\_id \downarrow,L\_key \downarrow, closest\_tuple \uparrow)$;	
				\State /*Adding $L\_t\_id$ into $j$'s $rvl$*/
				\State Append $L\_t\_id$ into $rvl$; 
				%                   \State \emph{unlock $x$};
				%                    \State return $(v)$; \Comment{v is the value returned}
				\If{$(closest\_tuple.m = TRUE)$}
				
				\State $L\_op\_status$ $\gets$ FAIL \label{lin:lookup18};
				\State $L\_val$ $\gets$ NULL \label{lin:lookup20};
				\Else
				\State $L\_op\_status$ $\gets$ OK;
				\State $L\_val$ $\gets$ $closest\_tuple.v$;
				\EndIf    
				%            \Else
				%                    \State /*Adding $i$ into $0$'s $rvl$*/
				%                    \State Append $i$ into $rvl$; 
				%                    \State $L\_op\_status$ $\gets$ FAIL;
				%                    \State $L\_val$ $\gets$ $NULL$;
				%\EndIf \label{lin:lookup30}

				\State $G\_pred.unlock()$;//$\Phi_{lp}$
				\State $G\_curr.unlock()$;
				\State    /*new log entry created to help upcoming method on the same key of the same tx*/
				\State $L\_rec$ $\gets$ Create new $L\_rec\langle L\_obj\_id, L\_key \rangle$\label{lin:lookup31}; 
				%\State ll.setPreds&Currs($obj\_id$ $\downarrow$, $key$ $\downarrow$, $preds[]$ $\downarrow$, $currs[]$ $\downarrow$);
				\State \llsval{$L\_val \downarrow$}
				\State \llspc{} \label{lin:lookup32};
			}						  
			
			%\EndIf \label{lin:lookup38}
			
			\EndIf \label{lin:lookup18}
			\cmnts{Update the local log} \label{lin:lookup19}
			\State \llsopn{$LOOKUP \downarrow$} \label{lin:lookup20};
			\State \llsopst{$L\_op\_status \downarrow$} \label{lin:lookup21};
			
			\State return $\langle L\_val, L\_op\_status\rangle$\label{lin:lookup22}; 
			
			\EndProcedure \label{lin:lookup23}
		\end{algorithmic}
		
%	\end{multicols}
	
\end{algorithm}

%%%%
%%%%%%%%%%%%%%%%%%%%%%%%%%%%%%%%%%%%%%%%%%%%%%%%%%%%%%%%%%%%%%%%%%%%%%
%-----------------------------------------STM\_DELETE-------------------------------------%------
%----
%%%%%%%%%%%%%%%%%%%%%%%%%%%%%%%%%%%%%%%%%%%%%%%%%%%%%%%%%%%%%%%%%%%%%%%%%%
%\begin{spacing}{2}
\begin{algorithm}[H]
%\algsetup{linenosize=\tiny}
\scriptsize
	\caption{\tabspace[0.2cm] STM $delete_{i}()$ : It will work same as a \npluk{}. If it is not the first method on a particular key means if its a subsequent method of the same transaction on that key then first it will search into the local log from \Lineref{delete3} to \Lineref{delete23}. If the previous method on the same key of same transaction was insert (from \Lineref{delete77} to \Lineref{delete10}) then \npdel{} will return the value based on previous operation value and status as OK and set the value and operation as NULL and DELETE respectively. 
    If previous method on the same key of same transaction was delete (from \Lineref{delete12} to \Lineref{delete15}) then \npdel{} will return the value and operation status as NULL and FAIL respectively.
    If previous method on the same key of same transaction was lookup (from \Lineref{delete16} to \Lineref{delete21}) then \npdel{} will return the value and operation status based on the previous operation value and status. If \npdel{} is the first method on that key (from \Lineref{delete24} to \Lineref{delete30}) then it will identify the location of node corresponding to the key in underlying DS with the help of \nplsls{} inside the \npcld{} method at \Lineref{delete25}.}
		%\emph{DESCP}\tabspace: If the Tx has locally done an operation returns apt value and status else does TO \tabspace[2.2cm] and method validation traversal phase in only.\\
		%\emph{IN}\tabspace \tabspace[0.72cm]: $obj\_id$, $key$\\
		%\emph{OUT}\tabspace \tabspace[0.37cm]: $value$, $op\_status$     }
	\label{algo:delete}
	\setlength{\multicolsep}{0pt}
%	\begin{multicols}{2}
	
	\begin{algorithmic}[1]
	\makeatletter\setcounter{ALG@line}{132}\makeatother
		\Procedure{STM delete}{$L\_t\_id \downarrow, L\_obj\_id \downarrow, L\_key \downarrow, L\_val \uparrow, L\_op\_status \uparrow$} \label{lin:delete1}
		%\State $op\_status$ $\gets$ RETRY \label{lin:lookup2};
			\cmnts{First identify the node corresponding to the key into local log}\label{lin:delete2}
		\If{$($\txlfind$)$} \label{lin:delete3}
	    \cmnts{Getting the previous operation's name}\label{lin:delete4}
			\State $L\_opn$ $\gets$ \llgopn{} ;\label{lin:delete5} %\Comment{$\Phi_{lp}$}
		\cmnts{If previous operation is insert then get the value based on the previous operations value and set the value and operation name as NULL and DELETE respectively}\label{lin:delete6}
		\If{$($\textup{INSERT} $=$ \textup{$L\_opn$}$)$} \label{lin:delete77}
		\State $L\_val$ $\gets$ \llgval{} \label{lin:delete7};
		
		\State \llsval{NULL $\downarrow$} \label{lin:delete8};

		\State \llsopn{DELETE $\downarrow$} \label{lin:delete9};
		
		\State $L\_op\_status$ $\gets$ OK \label{lin:delete10};
		\cmnts{If previous operation is delete then set the value as NULL}\label{lin:delete11}
		\ElsIf{$($\textup{DELETE} $=$ \textup{$L\_opn$}$)$} \label{lin:delete12}
		\State \llsval{NULL $\downarrow$} \label{lin:delete13};
		\State $L\_val$ $\gets$ NULL \label{lin:delete14}; 
		\State $L\_op\_status$ $\gets$ FAIL \label{lin:delete15}; 
		\Else \label{lin:delete16}
		
		\cmnts{If previous operation is lookup then get the value based on the previous operations value and set the value and operation name as NULL and DELETE respectively}\label{lin:delete17}
		\State $L\_val$ $\gets$ \llgval{} \label{lin:delete18}; 
		
		\State \llsval{NULL$ \downarrow$} \label{lin:delete19};

		\State \llsopn{DELETE $\downarrow$} \label{lin:delete20};
		\State $L\_op\_status$ $\gets$  $L\_rec.getOpStatus$($L\_obj\_id \downarrow$, $L\_key \downarrow$) \label{lin:delete21};
		
		\EndIf \label{lin:delete22}
		
		\Else \label{lin:delete23}

	%	\EndIf 
		    \cmnts{Common function for \rvmt{}, if node corresponding to the key is not part of local log}\label{lin:delete24}
			\State \cld{};		\label{lin:delete25}
		\EndIf \label{lin:delete26}
		\cmnts{Update the local log}\label{lin:delete27}
		\State \llsopn{$DELETE \downarrow$} ;\label{lin:delete28}
			\State \llsopst{$L\_op\_status \downarrow$} ;\label{lin:delete29}
			
			\State return $\langle L\_val, L\_op\_status\rangle$; \label{lin:delete30}
				
	\EndProcedure\label{lin:delete31}
	\end{algorithmic}
	
%	\end{multicols}
	
\end{algorithm}
\cmnt{
\begin{figure}[H]
	\captionsetup{justification=centering}
	%\includegraphics[scale=0.7]{figs/ex1.pdf_t}
	%\centerline{\scalebox{0.7}{\input{ex1.pstex_t}}}
	\centerline{\scalebox{0.38}{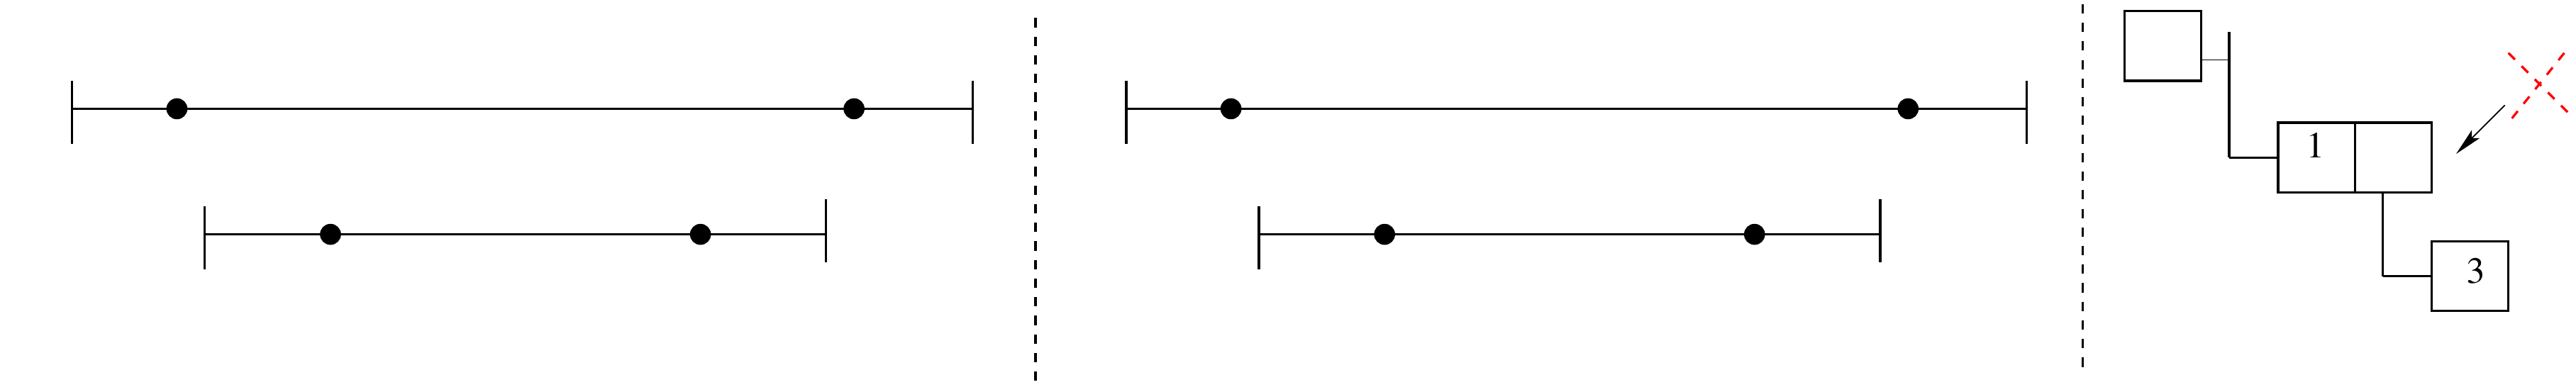}}
	\caption{Need of inserting $0^{th}$ version by \rvmt{} to satisfy opacity}
	\label{fig:mvostm8}
\end{figure}	
}
\begin{figure}[H]
	%\includegraphics[scale=0.7]{figs/ex1.pdf_t}
	%\centerline{\scalebox{0.7}{\input{ex1.pstex_t}}}
	\centerline{\scalebox{0.35}{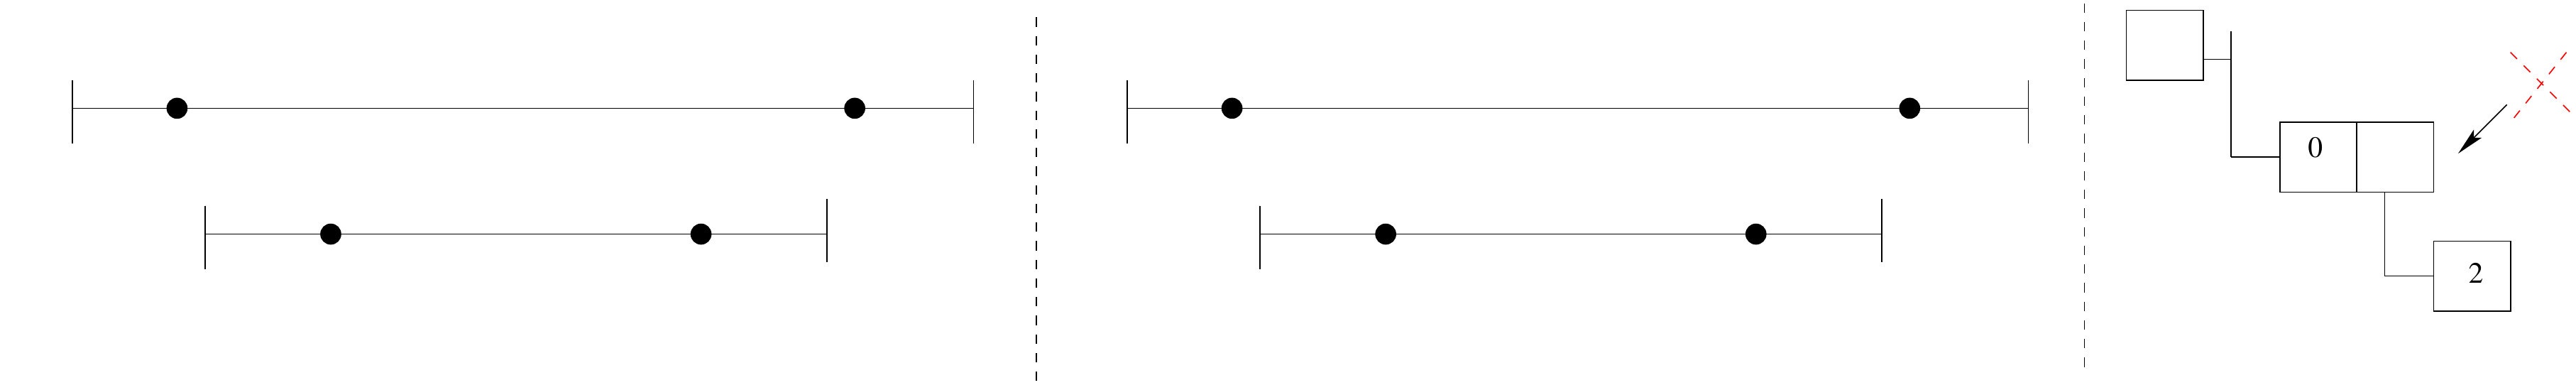}}
	\caption{Need of inserting $0^{th}$ version by \rvmt{} to satisfy opacity}
	\label{fig:mvostm8}
\end{figure}

%%%%%%%%%%%%%%%%%%%%%%%%%%%%%%%%%%%%%%%%%%%%%%%%%%%%%%%%%%%%%%%%%%%%%%%%%%
%-----------------------------------------commonLu\&Del-------------------------------------%------
%----
%%%%%%%%%%%%%%%%%%%%%%%%%%%%%%%%%%%%%%%%%%%%%%%%%%%%%%%%%%%%%%%%%%%%%%%%%%
%\begin{spacing}{2}
\begin{algorithm}[H]
%\algsetup{linenosize=\tiny}
%\scriptsize
	\caption{\tabspace[0.2cm] $commonLu\&Del()$ : This method is invoked by a \rvmt{} (\npluk{} and \npdel{}$)$, if node corresponding to the key is not part of local log. At \Lineref{com3} it identify the $\preds$ and $\currs$ for the node corresponding to the key in underlying DS with the help of \nplsls{}. If node corresponding to the key is in \bn{} of underlying DS then (from \Lineref{com5} to \Lineref{com17}) it finds the version tuple corresponding to the key which is having the largest timestamp less than itself as $closest\_tuple$ at \Lineref{com7}. After that, it will add itself into $closest\_tuple.rvl$ at \Lineref{com9}. If identified version mark field is TRUE then it will set the $L\_op\_status$ and $L\_val$ as FAIL and NULL otherwise, OK and value of identified tuple from \Lineref{com11} to \Lineref{com17} respectively. If node corresponding to the key is in \rn{} of underlying DS then (from \Lineref{scom5} to \Lineref{scom17}) it finds the version tuple corresponding to the key which is having the largest timestamp less than itself as $closest\_tuple$ at \Lineref{scom7}. After that, it will add itself into $closest\_tuple.rvl$ at \Lineref{scom9}. If identified version mark field is TRUE then it will set the $L\_op\_status$ and $L\_val$ as FAIL and NULL otherwise, OK and value of identified tuple from \Lineref{scom11} to \Lineref{scom17} respectively. 
	If node corresponding to the key is not part of underlying DS then (from \Lineref{com19} to \Lineref{com27}) it will create the new node corresponding to the key and add it into \rn{} of underlying DS with the help of \nplslins{} at \Lineref{com20}. After that it creates the $0^{th}$ version (at \Lineref{com22}) and add itself into $0^{th}.rvl$ at \Lineref{com23}. Then, it will set the $L\_op\_status$ and $L\_val$ as FAIL and NULL respectively at \Lineref{com25} and \Lineref{com26}. Finally, it will release the lock which is acquired in \nplsls{} at \Lineref{com3} and update the local log to help the upcoming method of the same transaction on the same key. \textbf{Why do we need to create a $0^{th}$ version by \rvmt{} in \rn{}?} This will be clear by the \figref{mvostm8}, where we have two concurrent transactions $T_1$ and $T_2$. History in the \figref{mvostm8}.a) is not opaque because we can't come up with any serial order. To make it serial (or opaque) first method $lu_2(ht, k_3, NULL)$ of transaction $T_2$ have to create the $0^{th}$ version in \rn{} if its not present in the underlying DS and add itself into $0^{th}.rvl$. So in future if any lower timestamp transaction less than $T_2$ will come then that lower transaction will ABORT (in this case transaction $T_1$ is aborting in (\figref{mvostm8}.b))) because higher timestamp already present in the $rvl$ (\figref{mvostm8}.c)) of the same version. After aborting $T_1$ we will get the serial history.}
	\scriptsize
\setlength{\multicolsep}{0pt}
%\begin{multicols}{2}
	
	\label{algo:commonlu&del}
%	\setlength{\multicolsep}{0pt}
%	\begin{multicols}{2}
	
	\begin{algorithmic}[1]
	\makeatletter\setcounter{ALG@line}{164}\makeatother
		\Procedure{commonLu\&Del}{$L\_t\_id \downarrow, L\_obj\_id \downarrow, L\_key \downarrow, L\_val \uparrow, L\_op\_status \uparrow$} \label{lin:com1} %\label{lin:commonlu&del}
		%\State $op\_status$ $\gets$ RETRY \label{lin:lookup2};
    \cmnts{If node corresponding to the key is not present in local log then search into underlying DS with the help of list\_lookup} \label{lin:com2}
			\State \lsls{}\label{lin:com3};
			\cmnts{ If node corresponding to the key is part of \bn{}}\label{lin:com4}
			\If{$(\bc.key = L\_key)$}\label{lin:com5}
						\cmnts{From $\bc.vls$, identify the right $version\_tuple$} \label{lin:com6}
                    \State \find($L\_t\_id \downarrow,\bc \downarrow, closest\_tuple \uparrow)$;\label{lin:com7}
                    
                    \cmnts{ Closest\_tuple is $\langle j,val,mark,rvl,vnext \rangle$} \label{lin:com8}

                    \State Adding $L\_t\_id$ into $j$'s $rvl$; \label{lin:com9}
                    %\State Append $L\_t\_id$ into $rvl$; 
 %                   \State \emph{unlock $x$};
%                    \State return $(v)$; \Comment{v is the value returned}
\cmnts{If the $closest\_tuple$ mark field is TRUE then $L\_op\_status$ and $L\_val$ set as FAIL and NULL otherwise set OK and value of $closest\_tuple$ respectively}\label{lin:com10}
                \If{$(closest\_tuple.mark = TRUE)$}\label{lin:com11}
                    
                    \State $L\_op\_status$ $\gets$ FAIL \label{lin:com12};
                    \State $L\_val$ $\gets$ NULL \label{lin:com13};
                \Else\label{lin:com14}
                    \State $L\_op\_status$ $\gets$ OK;\label{lin:com15}
                    \State $L\_val$ $\gets$ $closest\_tuple.val$; \label{lin:com16}
                \EndIf    \label{lin:com17}
        \cmnts{If node corresponding to the the key is part of \rn }
			\ElsIf{$(\rc.key = L\_key)$}\label{lin:scom5}
						\cmnts{From $\rc.vls$, identify the right $version\_tuple$} \label{lin:scom6}
                    \State \find($L\_t\_id \downarrow,\rc \downarrow, closest\_tuple \uparrow)$;\label{lin:scom7}
                    
                    \cmnts{Closest\_tuple is $\langle j,val,mark,rvl,vnext \rangle$} \label{lin:scom8}
\algstore{myalg}
\end{algorithmic}
\end{algorithm}

\begin{algorithm}                     
	\begin{algorithmic} [1]                   % enter the algorithmic environment
			\scriptsize
		\algrestore{myalg}
                    \State Adding $L\_t\_id$ into $j$'s $rvl$; \label{lin:scom9}
                    %\State Append $L\_t\_id$ into $rvl$; 
 %                   \State \emph{unlock $x$};
%                    \State return $(v)$; \Comment{v is the value returned}
\cmnts{If the $closest\_tuple$ mark field is TRUE then $L\_op\_status$ and $L\_val$ set as FAIL and NULL otherwise set OK and value of $closest\_tuple$ respectively}\label{lin:scom10}
                \If{$(closest\_tuple.mark = TRUE)$}\label{lin:scom11}
                    
                    \State $L\_op\_status$ $\gets$ FAIL \label{lin:scom12};
                    \State $L\_val$ $\gets$ NULL \label{lin:scom13};
                \Else\label{lin:scom14}
                    \State $L\_op\_status$ $\gets$ OK;\label{lin:scom15}
                    \State $L\_val$ $\gets$ $closest\_tuple.val$; \label{lin:scom16}
                \EndIf    \label{lin:scom17}

        \Else\label{lin:com18}
        		\cmnts{If node corresponding to the key is not part of \rn as well as \bn then create the node into \rn with the help of list\_Ins()}\label{lin:com19}
		        \State \lslins{$RL \downarrow$};\label{lin:com20}
		        \cmnts{Insert the $0^{th}$ version tuple} \label{lin:com21}
		        \State insert $v\_tuple \langle 0,NULL,T,NULL,NULL \rangle$ into $node.vl$ in the increasing order;	 \label{lin:com22}
                  \State Adding $L\_t\_id$ into $0^{th}.rvl$;\label{lin:com23}
                    %\State Append $L\_t\_id$ into $rvl$;
                \cmnts{Setting $L\_op\_status$ and $L\_val$ as FAIL and NULL because its reading from the marked version, which is TRUE}\label{lin:com24}    
                \State    $L\_op\_status$ $\gets$ FAIL ;\label{lin:com25}
                    \State $L\_val$ $\gets$ NULL ;\label{lin:com26}
			\EndIf\label{lin:com27}
			\cmnts{Releasing the locks in increasing order}\label{lin:com28}
			  	    \State releasePred\&CurrLocks($ \preds \downarrow$, $ \currs \downarrow$);
\cmnts{Create local log record and append it into increasing order of keys}\label{lin:com31}						\State $L\_rec$ $\gets$ Create new $L\_rec\langle L\_obj\_id, L\_key \rangle$\label{lin:com32}; 
						%\State ll.setPreds&Currs($obj\_id$ $\downarrow$, $key$ $\downarrow$, $preds[]$ $\downarrow$, $currs[]$ $\downarrow$);
						\State \llsval{$L\_val \downarrow$} \label{lin:com33}
						\State \llspc{} ;

			\State return $\langle L\_val, L\_op\_status\rangle$;\label{lin:com34}
				
	\EndProcedure 
	\end{algorithmic}
	
%	\end{multicols}
	
\end{algorithm}

%%%%%%%%%%%%%%%%%%%%%%%%%%%%%%%%%%%%%%%%%%%%%%%%%%%%%%%%%%%%%%%%%%%%%%%%%%
%-----------------------------------------TryCommit----------------------------------%---------
%----
%%%%%%%%%%%%%%%%%%%%%%%%%%%%%%%%%%%%%%%%%%%%%%%%%%%%%%%%%%%%%%%%%%%%%%%%%%

\begin{algorithm}[H]
\scriptsize
	\caption{\tabspace[0.2cm] STM $tryC()$ : The actual effect of \upmt{s} (\npins{} and \npdel{}) will take place in \nptc{} method. From \Lineref{tryc5} to \Lineref{tryc15} will identify and validate the $\preds$ and $\currs$ of each \upmt{} of same transaction. At \Lineref{tryc9} it will validate if there exist any higher timestamp transaction in the $rvl$ of the $closest\_tuple$ of $\bc$ then returns ABORT at \Lineref{tryc11}. Same as at \Lineref{stryc9} it will validate if there exist any higher timestamp transaction in the $rvl$ of the $closest\_tuple$ of $\rc$ then returns ABORT at \Lineref{stryc11}. Otherwise it will perform the above steps for remaining \upmt{s}. On successful validation of all the \upmt{s}, the actually effect will be taken place from \Lineref{tryc17} to \Lineref{tryc43}. If the \upmt{} is insert and node corresponding to the key is part of \bn{} then it creates the new version tuple and add it in increasing order of version list from \Lineref{tryc22} to \Lineref{tryc24}. If node corresponding to the key is part of \rn{} then it adds the same node in the \bn{} as well with the help of \nplslins{} at \Lineref{stryc24} and creates the new version tuple and add it in increasing order of version list from \Lineref{stryc23} to \Lineref{stryc25}. Otherwise it will create the node and insert it into \bn{} with the help of \nplslins{} and insert the version tuple from \Lineref{tryc25} to \Lineref{tryc29}. If the \upmt{} is delete and node corresponding to the key is part of \bn{} then it creates the new version tuple and set its mark field as TRUE and add it in increasing order of version list from \Lineref{tryc31} to \Lineref{stryc35}. After successful completion of each \upmt{}, it will validate the $\preds$ and $\currs$ of upcoming \upmt{} of the same transaction with the help of \npintv{} at \Lineref{tryc42}. Eventually, it will release all the locks at \Lineref{tryc45} in the same order of lock acquisition.} %: All update methods will takes effect in underlying data-structure atomically if the validation will succeed. 
		%\emph{DESCP}\tabspace: All update methods of the transaction take ordered locks, validate and update underlying \tabspace[2.2cm]  data-structure atomically. \\
		%\emph{IN}\tabspace \tabspace[0.72cm]: \\
		%\emph{OUT}\tabspace \tabspace[0.37cm]: $txstatus$     }
	\label{algo:trycommit}
	\setlength{\multicolsep}{0pt}
%		\begin{multicols}{2}
	\begin{algorithmic}[1]
\makeatletter\setcounter{ALG@line}{213}\makeatother
		\Procedure{STM tryC}{$L\_t\_id \downarrow, L\_tx\_status \uparrow$} \label{lin:tryc1}

%\State    /*get the tx id*/
%		\State $L\_t\_id$ $\gets$ getTS($t_i \downarrow$) \label{lin:tryc2};
		\cmnts{Get the local log list corresponding to each transaction which is in increasing order of keys}\label{lin:tryc2}
		\State $L\_list$ $\gets$ $L\_txlog.getList$($L\_t\_id \downarrow$) \label{lin:tryc3};
%		\State    /*sort the local log in increasing order of keys and copy into ordered list*/
%		\State $L\_ordered$ $\gets$ \llsort{} \label{lin:tryc4};
\cmnts{Identify the new $\preds$ and $\currs$ for all update methods of a transaction and validate it}\label{lin:tryc4}
		\While{$(\textbf{$L\_rec_{i} \gets \textup{next}(L\_list$}))$} \label{lin:tryc5}
		\State ($L\_key, L\_obj\_id$) $\gets$ \llgkeyobj{} \label{lin:tryc6};
		\cmnts{Identify the new $G\_pred$ and $G\_curr$ location with the help of list\_lookup()}\label{lin:tryc7}
		\State \lsls{$COMMIT \downarrow$} \label{lin:tryc8};
			
		\If {$((\bc.key = L\_key) \& (\checkv(L\_t\_id \downarrow,\bc \downarrow) = FALSE))$}\label{lin:tryc9}
%\State $\remid(i)$;
\State Unlock all the variables;\label{lin:tryc10}
\State return $ABORT$;\label{lin:tryc11}
\ElsIf {$((\rc.key = L\_key) \& (\checkv(L\_t\_id \downarrow,\rc \downarrow) = FALSE))$}\label{lin:stryc9}
%\State $\remid(i)$;
\State Unlock all the variables;\label{lin:stryc10}
\State return $ABORT$;\label{lin:stryc11}

\EndIf;\label{lin:tryc12}

					%State    /*if list\_lookup return op\_status as ABORT then method will return ABORT*/
		%If{$(op\_status_{ll}$ $=$ \textup{ABORT}$)$} \label{lin:tryc8}
%		\State release all the locks
		%State \handlea{} \label{lin:tryc9};
		
		%\State return \label{lin:tryc10};
		
		%EndIf \label{lin:tryc11}
			\cmnts{Update the log entry} \label{lin:tryc13}

		\State \llspc{} \label{lin:tryc14};
		\EndWhile \label{lin:tryc15}
	\cmnts{Get each update method one by one and take effect in underlying DS}\label{lin:tryc16}
		\While{$(\textbf{$L\_rec_{i} \gets \textup{next}(L\_list$}))$} \label{lin:tryc17}
		\State ($L\_key, L\_obj\_id$) $\gets$ \llgkeyobj{} \label{lin:tryc18};
		\cmnts{Get the operation name from local log record}\label{lin:tryc19}
		\State $L\_opn$ $\gets$ $(L\_rec)_{i}$.$L\_opn$ \label{lin:tryc20};
		
					\cmnts{Modify the $\preds$ and $\currs$ for the consecutive update methods which are working on overlapping zone in lazy-list}\label{lin:tryc41}
		\State intraTransValdation($L\_rec_{i} \downarrow$, $\preds \uparrow$, $\currs \uparrow$) \label{lin:tryc42};
\cmnts{If operation is insert then after successful completion of it node corresponding to the key should be part of \bn}\label{lin:tryc21}
\algstore{myalg}
\end{algorithmic}
\end{algorithm}

\begin{algorithm}                     
	\begin{algorithmic} [1]                   % enter the algorithmic environment
			\scriptsize
		\algrestore{myalg}
		\If{$($\textup{INSERT} $=$ \textup{$L\_opn$}$)$} \label{lin:tryc22}
	%\State    /*if node corresponding to the key is part of \bn*/
		\If{$(\bc.key) = L\_key)$} \label{lin:tryc23}
	\State insert $v\_tuple \langle L\_t\_id,val,F,NULL,NULL \rangle$ into $G\_curr.vl$ in the increasing order;	\label{lin:tryc24}
	
	\ElsIf{$(\rc.key) = L\_key)$} \label{lin:stryc23}
	\State \lslins{$RL\_BL \downarrow$} \label{lin:stryc24}
	\State insert $v\_tuple \langle L\_t\_id,val,F,NULL,NULL \rangle$ into $G\_curr.vl$ in the increasing order;	\label{lin:stryc25}
	
		\Else \label{lin:tryc25}
		\cmnts{If node corresponding to the key is not part underlying DS then create the node with the help of list\_Ins() and insert it into \bn}\label{lin:tryc26}
		\State \lslins{$BL \downarrow$} \label{lin:tryc27};
		\State insert $v\_tuple \langle L\_t\_id,val,F,NULL,NULL \rangle$ into $node.vl$ in the increasing order;	\label{lin:tryc28}
%	\State    /*set the op\_status as OK in local log*/
%		\State \llsopst{$OK \downarrow$} \label{lin:tryc30};
	%\State    /*update the max\_ts of insert for node corresponding to the key into underlying DS*/		
	%	\State $\texttt{write}$(node.max\_ts.insert, TS($t_i$)) \label{lin:tryc31};
		\EndIf \label{lin:tryc29}
		\cmnts{If operation is delete then after successful completion of it node corresponding to the key should part of \rn only}\label{lin:tryc30}
		\ElsIf{$($\textup{DELETE} $=$ $L\_opn)$} \label{lin:tryc31}
	\cmnts{If node corresponding to the key is part of \bn}\label{lin:tryc32}

		\If{$(\bc.key) = L\_key)$} \label{lin:tryc33}
	%\State    /*delete the node corresponding to the key from the \bn with the help of lslDel()*/	
			\State insert $v\_tuple \langle L\_t\_id,NULL,T,NULL,NULL \rangle$ into $G\_curr.vl$ in the increasing order;	\label{lin:tryc34}
			\State \lsldel{} \label{lin:stryc35};
%		\State    /*set the op\_status as OK in local log*/
%		\State \llsopst{$OK \downarrow$} \label{lin:tryc36};
		%\State    /*update the max\_ts of delete for node corresponding to the key into underlying DS*/	
		%\State $\texttt{write}$(\textcolor{blue}{$currs[1]$}.max\_ts.delete, TS($t_i$)) \label{lin:tryc37};
\cmnt{
		\Else \label{lin:tryc35}
		\State    /*If node corresponding to the key is not part underlying DS then create the node with the help of list\_Ins() */\label{lin:tryc36}
		\State \lslins{$RL \downarrow$};\label{lin:tryc37}
		
		\State insert $v\_tuple \langle L\_t\_id,NULL,T,NULL,NULL \rangle$ into $node.vl$ in the increasing order;	\label{lin:tryc38}
		%\State \llsopst{$FAIL \downarrow$} \label{lin:tryc39};
		
		%\State $write$(\textcolor{red}{$currs[0]$}.max\_ts.delete, TS($t_i$)) \label{lin:tryc40};
}	
		\EndIf \label{lin:tryc39}
	
		\EndIf \label{lin:tryc40}

		\EndWhile \label{lin:tryc43}
		\cmnts{Release all the locks in increasing order}\label{lin:tryc44}
		\State \rlsol{} \label{lin:tryc45};  
		\cmnts{Set the transaction status as OK}\label{lin:tryc46}
		\State $L\_tx\_status$ $\gets$ OK \label{lin:tryc47};
%		
%		\State \txsetst{} \label{lin:tryc46};
		\State return $\langle L\_tx\_status\rangle$\label{lin:tryc48};
		\EndProcedure \label{lin:tryc49}
	\end{algorithmic}
%		\end{multicols}
\end{algorithm}

	%%%%%%%%%%%%%%%%%%%%%%%%%%%%%%%%%%%%%%%%%%%%%%%%%%%%%%%%%%%%%%%%%%%%%%%%%%
	%------------------- lazyrblist-delete -----------------------
	%%%%%%%%%%%%%%%%%%%%%%%%%%%%%%%%%%%%%%%%%%%%%%%%%%%%%%%%%%%%%%%%%%%%%%%%%%
	
	\begin{algorithm}[H]
		\scriptsize
		\caption{\tabspace[0.2cm] \dell() : Delete a node from blue link in underlying hash table at location corresponding to $\preds$ \& $\currs$.}
			%\emph{DESCP}\tabspace: Deletes a node from blue list in underlying hash table at location corresponding to \tabspace[2.2cm] preds[] \& currs[].\\
			%\emph{IN}\tabspace \tabspace[0.72cm]: $preds[], currs[]$  \\
			%\emph{OUT}\tabspace \tabspace[0.37cm]:  }
		\label{algo:lsldelete}
		\setlength{\multicolsep}{0pt}
%		\begin{multicols}{2}
			\begin{algorithmic}[1]
				\makeatletter\setcounter{ALG@line}{265}\makeatother
				\Function{list\_del}{$\preds \downarrow, \currs \downarrow$} \label{lin:lsldel1}
				
				%\cmnts{mark the node$ \langle obj\_id, key \rangle$ for deletion}
				%\State $\texttt{write}$($\bc$.marked, True) \label{lin:lsldel2};
				\cmnts{Update the blue links}
				\State $\bp$.\bn $\gets$ $\bc$.\bn \label{lin:lsldel3};
				\State return $\langle void \rangle$;
				\EndFunction \label{lin:lsldel4}
			\end{algorithmic}
			
%		\end{multicols}
	\end{algorithm}

%%%%%%%%%%%%%%%%%%%%%%%%%%%%%%%%%%%%%%%%%%%%%%%%%%%%%%%%%%%%%%%%%%%%%%%%%%
%----------------- List lookup() ---------------------------
%%%%%%%%%%%%%%%%%%%%%%%%%%%%%%%%%%%%%%%%%%%%%%%%%%%%%%%%%%%%%%%%%%%%%%%%%%
%\begin{spacing}{0.8}
\begin{algorithm}[H]
\scriptsize
%lslSearch($obj\_id \downarrow, key \downarrow, preds[] \uparrow, currs[] \uparrow, value \uparrow, val\_type \downarrow$)
	\caption{list\_lookup() : This method is called by \rvmt{} and \upmt{}. It finds the location of the node corresponding to the key in underlying DS from \Lineref{lslsearch5} to \Lineref{slslsearch15}. First it identifies the node in \bn{} (from \Lineref{lslsearch5} to \Lineref{lslsearch15}) then in \rn{} (from \Lineref{slslsearch9} to \Lineref{slslsearch15}). After finding the appropriate location of the node corresponding to the key in the form of $\preds$ and $\currs$, it will acquire the locks on it at \Lineref{lslsearch17} and validate it at \Lineref{lslsearch20}.}
		%\emph{DESCP}\tabspace: Finds location of the corresponding $\left\langle obj\_id, key  \right\rangle$ in underlying hash table. color of preds[] \tabspace[2.2cm] \& currs[] depicts the red or blue node.\\
		%\emph{IN}\tabspace \tabspace[0.72cm]: $\left\langle obj\_id, key  \right\rangle$, $val\_type$  \\
		%\emph{OUT}\tabspace \tabspace[0.37cm]: $preds[], currs[], value$     }
	\label{algo:lslsearch}
	\setlength{\multicolsep}{0pt}
%		\begin{multicols}{2}
	\begin{algorithmic}[1]
	\makeatletter\setcounter{ALG@line}{270}\makeatother	
		\Procedure{list\_lookup}{$L\_obj\_id \downarrow, L\_key \downarrow, G\_preds[] \uparrow, G\_currs[] \uparrow$} \label{lin:lslsearch1}

	\cmnts{By default setting the $L\_op\_status$ as RETRY}\label{lin:lslsearch2}
	    \State STATUS $L\_op\_status$ $\gets$ RETRY; \label{lin:lslsearch3}
	 \cmnts{Identify the \preds and \currs for node corresponding to the key if $L\_op\_status$ is RETRY}\label{lin:lslsearch4}   
		\While{($L\_op\_status$ = \textup{RETRY})} \label{lin:lslsearch5}
		\cmnts{Get the head of the bucket in chaining hash-table with the help of $L\_obj\_id$ and $L\_key$}\label{lin:lslsearch6}
		\State $G\_head$ $\gets$ \glslhead \label{lin:lslsearch7};
		\cmnts{Initialize $\bp$ to head}\label{lin:lslsearch8}
		\State $\bp$ $\gets$ $G\_head$ \label{lin:lslsearch9}; 
		\cmnts{Initialize $\bc$ to $\bp.\bn$}\label{lin:lslsearch10}
		\State $\bc$ $\gets$ $\bp.\bn$ \label{lin:lslsearch11};
		\cmnts{Searching node corresponding to the key into \bn}
		\While{$((\bc.key) < L\_key)$} \label{lin:lslsearch12}
		\State $\bp$ $\gets$ $\bc$ \label{lin:lslsearch13};
				
		\State $\bc$ $\gets$ $\bc.\bn$ \label{lin:lslsearch14};
			
		\EndWhile \label{lin:lslsearch15}
		
		\cmnts{Initialize $\rp$ to head}\label{lin:slslsearch8}
		\State $\rp$ $\gets$ $\bp$ \label{lin:slslsearch9}; 
		\cmnts{Initialize $\rc$ to $\rp.\rn$}\label{lin:slslsearch10}
		\State $\rc$ $\gets$ $\rp.\rn$ \label{lin:slslsearch11};
		\cmnts{Searching node corresponding to the key into \rn}
		\While{$((\rc.key) < L\_key)$} \label{lin:slslsearch12}
		\State $\rp$ $\gets$ $\rc$ \label{lin:slslsearch13};
				
		\State $\rc$ $\gets$ $\rc.\rn$ \label{lin:slslsearch14};
			
		\EndWhile \label{lin:slslsearch15}

		%\State    /*get the value*/
		%\State $L\_val$ $\gets$ $G\_curr.value$
		\cmnts{Acquire the locks on increasing order of keys}\label{lin:lslsearch16}
	    \State acquirePred\&CurrLocks($ \preds \downarrow$, $ \currs \downarrow$); \label{lin:lslsearch17}
\cmnts{Method validation to identify the changes done by concurrent conflicting method}\label{lin:lslsearch19}
		\State methodValidation($\preds$ $\downarrow$, $\currs$ $\downarrow$, $L\_op\_status \uparrow$)\label{lin:lslsearch20};	
		%\State $op\_status$ $\gets$ \validation \label{lin:lslsearch21};
\cmnts{If $L\_op\_status$ is RETRY then release all the locks}		\label{lin:lslsearch21}
		\If{(($L\_op\_status$ = \textup{RETRY}))} \label{lin:lslsearch22}
	    \State releasePred\&CurrLocks($ \preds \downarrow$, $ \currs \downarrow$);
	    \EndIf \label{lin:lslsearch25}
			
		\EndWhile \label{lin:lslsearch26}
		
		\State return $\langle G\_preds[], G\_currs[]\rangle$ \label{lin:lslsearch27};
	
	\EndProcedure \label{lin:lslsearch28}
	\end{algorithmic}
%		\end{multicols}
\end{algorithm}
%\end{spacing}

%%%%%%%%%%%%%%%%%%%%%%%%%%%%%%%%%%%%%%%%%%%%%%%%%%%%%%%%%%%%%%%%%%%%%%%%%%
	%------------------- acquirepreds&currs -----------------------
	%%%%%%%%%%%%%%%%%%%%%%%%%%%%%%%%%%%%%%%%%%%%%%%%%%%%%%%%%%%%%%%%%%%%%%%%%%
	
	\begin{algorithm}[H]
		\scriptsize
		\caption{\tabspace[0.2cm] acquirePred\&CurrLocks() : acquire all locks taken during \nplsls{}.}
			%\emph{DESCP}\tabspace: releases all locks taken during tryCommit\\
			%\emph{IN}\tabspace \tabspace[0.72cm]: $ordered\_ll\_list$\\
			%\emph{OUT}\tabspace \tabspace[0.37cm]:   }
		\label{algo:acquirepreds&currs}
		\setlength{\multicolsep}{0pt}
%		\begin{multicols}{2}
			\begin{algorithmic}[1]
				\makeatletter\setcounter{ALG@line}{306}\makeatother
				\Function{acquirePred\&CurrLocks}{$ \preds \downarrow$, $ \currs \downarrow$}
				\State $\bp$.$\texttt{lock()}$;
				\State $\rp$.$\texttt{lock()}$;
				\State $\rc$.$\texttt{lock()}$;
				\State $\bc$.$\texttt{lock()}$;
				\State return $\langle void \rangle$;        
				\EndFunction
			\end{algorithmic}
			
%		\end{multicols}
	\end{algorithm}
	
	%%%%%%%%%%%%%%%%%%%%%%%%%%%%%%%%%%%%%%%%%%%%%%%%%%%%%%%%%%%%%%%%%%%%%%%%%%
	%------------------- releasepreds&currs -----------------------
	%%%%%%%%%%%%%%%%%%%%%%%%%%%%%%%%%%%%%%%%%%%%%%%%%%%%%%%%%%%%%%%%%%%%%%%%%%
	
	\begin{algorithm}[H]
		\scriptsize
		\caption{\tabspace[0.2cm] releasePred\&CurrLocks() : Release all locks taken during \nplsls{}.}
			%\emph{DESCP}\tabspace: releases all locks taken during tryCommit\\
			%\emph{IN}\tabspace \tabspace[0.72cm]: $ordered\_ll\_list$\\
			%\emph{OUT}\tabspace \tabspace[0.37cm]:    }
		\label{algo:releasepreds&currs}
		\setlength{\multicolsep}{0pt}
%		\begin{multicols}{2}
			\begin{algorithmic}[1]
				\makeatletter\setcounter{ALG@line}{313}\makeatother
				\Function{releasePred\&CurrLocks}{$ \preds \downarrow$, $ \currs \downarrow$}
				\State $\bp$.$\texttt{unlock()}$\label{lin:rpandc};//$\Phi_{lp}$ 
				\State $\rp$.$\texttt{unlock()}$;
				\State $\rc$.$\texttt{unlock()}$;
				\State $\bc$.$\texttt{unlock()}$;
				\State return $\langle void \rangle$;        
				\EndFunction
			\end{algorithmic}
			
%		\end{multicols}
	\end{algorithm}
	%\end{multicols}

%%%%%%%%%%%%%%%%%%%%%%%%%%%%%%%%%%%%%%%%%%%%%%%%%%%%%%%%%%%%%%%%%%%%%%%%%%
%----------------------------list-insert --------------------------------
%%%%%%%%%%%%%%%%%%%%%%%%%%%%%%%%%%%%%%%%%%%%%%%%%%%%%%%%%%%%%%%%%%%%%%%%%%

%\vspace{-.5cm}
\begin{algorithm}[H]
\scriptsize
	\caption{\tabspace[0.2cm] list\_Ins(): This method is called by the \rvmt{} and \upmt{}. Color of preds \& currs depicts the red or blue node.}
		%\emph{DESCP}\tabspace: Inserts or overwrites a node in underlying hash table at location corresponding to \tabspace[2.2cm] preds[] \& currs[]. Color of preds[] \& currs[] depicts the red or blue node.\\
		%\emph{IN}\tabspace \tabspace[0.72cm]: $preds[], currs[], list\_type$  \\
		%\emph{OUT}\tabspace \tabspace[0.37cm]:     }
	\label{algo:lslins}
		\setlength{\multicolsep}{0pt}
%	\begin{multicols}{2}
	\begin{algorithmic}[1]
\makeatletter\setcounter{ALG@line}{320}\makeatother
		\Procedure{list\_Ins}{$\preds \downarrow, \currs \downarrow, list\_type \downarrow, node \uparrow$} \label{lin:lslins1}

\cmnts{Inserting the node from redlist to bluelist}
				\If{$((list\_type)$ $=$ $($\textcolor{black}{$RL$}$\_$\textcolor{black}{$BL$}$))$} \label{lin:lslins2}
				
				%\State $\texttt{write}$($\rc$.marked, false) \label{lin:lslins3}; 
				\State $\rc$.\bn $\gets$ $\bc$ \label{lin:lslins4};
				\State $\bp$.\bn $\gets$ $\rc$ \label{lin:lslins5};
				\cmnts{Inserting the node into redlist only}
				\ElsIf{$((list\_type$) $=$ \textcolor{black}{$RL$}$)$} \label{lin:lslins6}
				\State node = Create new node()
				\label{lin:lslins7};
						\cmnts{After created the node acquiring the lock on it}\label{lin:lslins4}
		\State node.lock();\label{lin:lslins5}
		
				\State node.\rn $\gets$ $\rc$ \label{lin:lslins9};
				\State $\rp$.\rn $\gets$ node \label{lin:lslins10};
				
				\Else \label{lin:lslins11}
				\cmnts{Inserting the node into red as well as blue list}
				\State node = new node() \label{lin:lslins12}; %\Comment{default locked state for thread validation}
				\cmnts{After creating the node acquiring the lock on it}
				\State node.lock();
				\State node.\rn $\gets$ $\rc$ \label{lin:lslins13};
				\State node.\bn $\gets$ $\bc$ \label{lin:lslins14};
				
				\State $\rp$.\rn $\gets$ node \label{lin:lslins15};
				
				\State $\bp$.\bn $\gets$ node \label{lin:lslins16};
				\EndIf \label{lin:lslins17}
				\State return $\langle node \rangle$;
			
\cmnt{

        \State    /*Inserting the new node corresponding to the key into Underlying DS/\label{lin:lslins2}
		\State node = Create new node() \label{lin:lslins3}; %\Comment{default locked state for thread validation}
		\State    /*After created the node acquiring the lock on it*/\label{lin:lslins4}
		\State node.lock();\label{lin:lslins5}
		\State /*Adding the new node at appropriate location (in increasing order of the keys) with the help of $G\_pred$ and $G\_curr$*/\label{lin:lslins6}
		\State node.knext $\gets$ $G\_curr$ \label{lin:lslins7};
		\State $G\_pred$.knext $\gets$ node \label{lin:lslins8};
		\State return $\langle node \rangle$;\label{lin:lslins9}}
		\EndProcedure \label{lin:lslins10}
	\end{algorithmic}
%	\end{multicols}
\end{algorithm}

%%%%%%%%%%%%%%%%%%%%%%%%%%%%%%%%%% find_lts(largest timestamp but less then itself)   %%%%%%%%%%%%%%%%%%%%%%%%%%%%%%%%%%%%%% 
%%%%%%%%%%%%%%%%%%%%%%%%%%%%%%%%%%%%%%%%%%%%%%%%%%%%%%%%%%%%%%%%%%%%%%

\begin{algorithm}  
\scriptsize
\label{alg:select}
\caption{$\find()$: This method is called by \rvmt{} and \upmt{} to identify a  $closest\_tuple$ $\langle j,val,mark,rvl,vnext \rangle$ created by the transaction $T_j$ with the largest timestamp smaller than $L\_t\_id$ from \Lineref{findlts5} to \Lineref{findlts10}.}
		\setlength{\multicolsep}{0pt}
%	\begin{multicols}{2}
\begin{algorithmic}[1]
\makeatletter\setcounter{ALG@line}{344}\makeatother
\Procedure{find\_lts}{$L\_t\_id \downarrow, \currs \downarrow, closest\_tuple \uparrow$} \label{lin:findlts1}
\cmnts{Initialize $closest\_tuple$} \label{lin:findlts2}
\State $closest\_tuple = \langle 0,NULL,F,NULL,NULL \rangle$;\label{lin:findlts3}
\cmnts{For all the version of $\currs$ identify the largest timestamp less than $L\_t\_id$} \label{lin:findlts4}
\ForAll {$\langle p,val,mark,rvl,vnext \rangle \in \currs.vl$} \label{lin:findlts5}
\If {$(p < L\_t\_id)$ and $(closest\_tuple.ts < p)$} \label{lin:findlts6}
\cmnts{Assign closest tuple as $\langle p,val,mark,rvl,vnext \rangle$, if any version tuple is having largest timestamp less then L\_t\_id exist} \label{lin:findlts7}
\State $closest\_tuple = \langle p,val,mark,rvl,vnext \rangle$; \label{lin:findlts8}
\EndIf\label{lin:findlts9}
\EndFor\label{lin:findlts10}
\State return $\langle closest\_tuple\rangle$; \label{lin:findlts11}
\EndProcedure\label{lin:findlts12}
\end{algorithmic}
%\end{multicols}
\end{algorithm}

\begin{figure} [tbph]
	\captionsetup{justification=centering}
	%\centering
	%\includegraphics[scale=.5]{figs/fig3.png}
	%\includegraphics[scale=.5]{figs/fig3.pdf_t}
	\centerline{\scalebox{0.5}{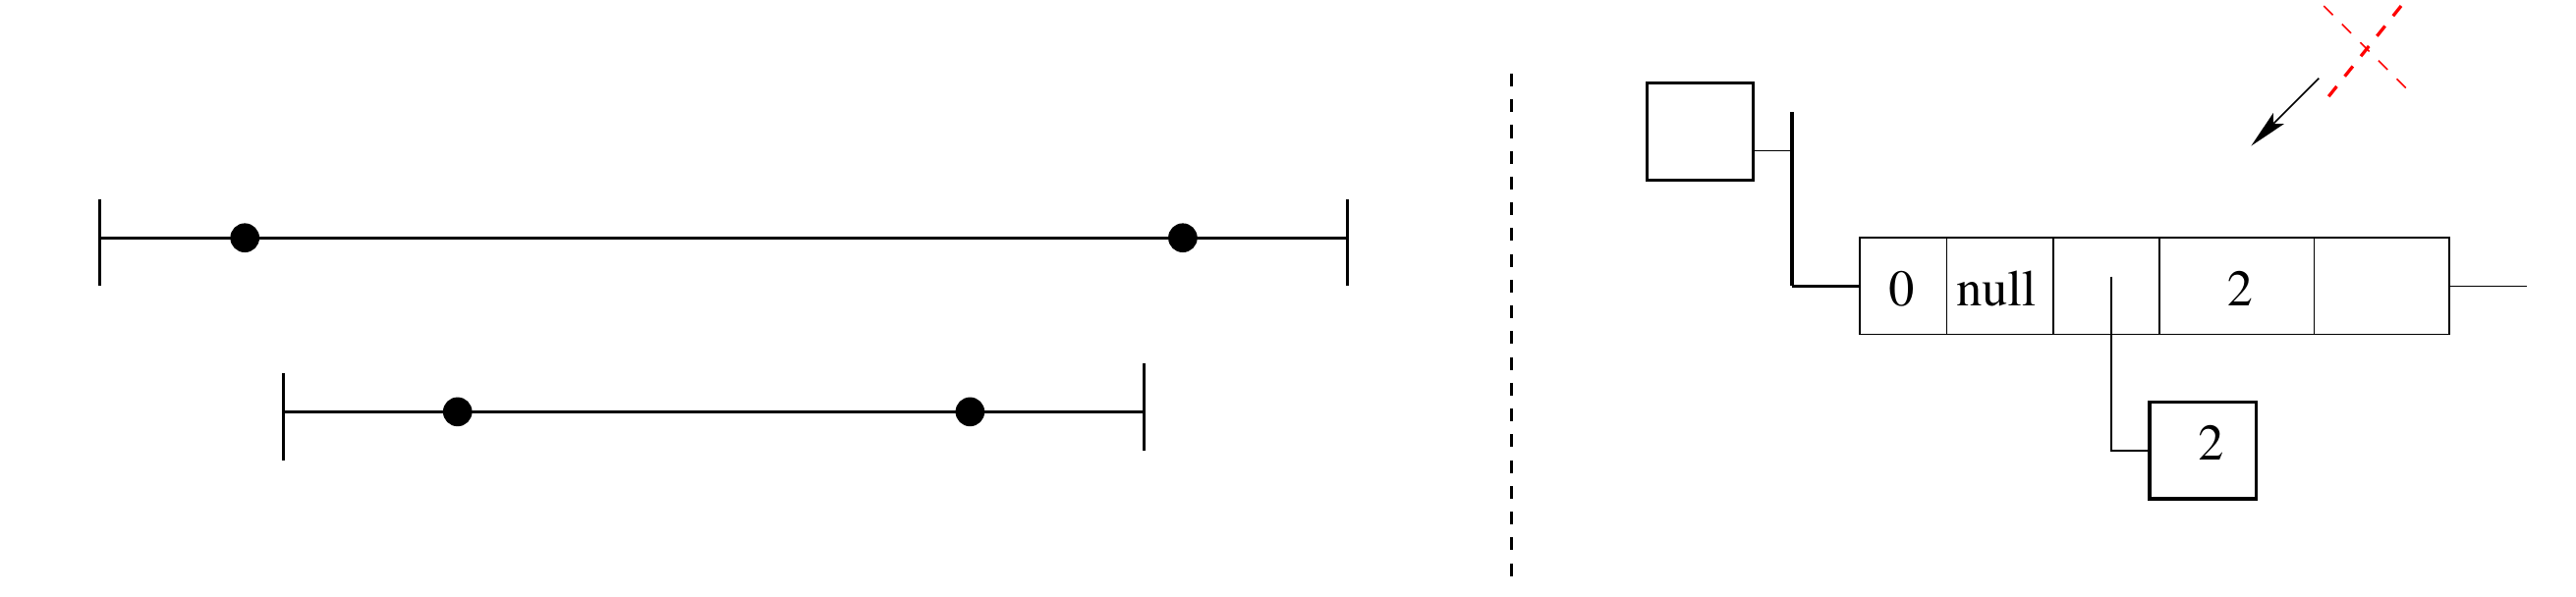}}
	\caption{Validation by $check\_version$}
	\label{fig:mvostmm12}
\end{figure}

\cmnt{
\begin{figure} [tbph]
	%\centering
	%\includegraphics[scale=.5]{figs/fig3.png}
	%\includegraphics[scale=.5]{figs/fig3.pdf_t}
	\centerline{\scalebox{0.5}{\input{figs/mvostm12.pdf_t}}}
	\caption{Validation by $check\_version$}
	\label{fig:mvostm12}
\end{figure}
}

%%%%%%%%%%%%%%%%%%%%%%%%%%%%%%%%%%%%%%%%%%%%%%%%%%%%%%%%%%%%%%%%%%%%%%%%%%
%---------------------------------Check Version -------------------
%%%%%%%%%%%%%%%%%%%%%%%%%%%%%%%%%%%%%%%%%%%%%%%%%%%%%%%%%%%%%%%%%%%%%%%%%%

\begin{algorithm}  
\scriptsize
\label{alg:checkVersion} 
\caption{$\checkv()$: This method is called by the \nptc{}. First it will find the $closest\_tuple$ $\langle j,val,mark,rvl,vnext \rangle$ created by the transaction $T_j$ with the largest timestamp smaller than $L\_t\_id$ at \Lineref{checkVersion3}. Then, it checks the version list to identify is there any higher timestamp already present in the $rvl$ of $closest\_tuple$ from \Lineref{checkVersion5} to \Lineref{checkVersion11}. If it presents then it will returns FALSE at \Lineref{checkVersion9} otherwise, TRUE at \Lineref{checkVersion13}. It will be more clear by the \figref{mvostmm12}.a) where second method $ins_1(ht, k_3, ABORT)$ of transaction $T_1$ will ABORT because higher transaction $T_2$ timestamp is already present in the $rvl$ of $closest\_tuple$ as $0^{th}$ version in \figref{mvostmm12}.b).}
		\setlength{\multicolsep}{0pt}
%	\begin{multicols}{2}
\begin{algorithmic}[1]
\makeatletter\setcounter{ALG@line}{356}\makeatother
\Procedure{check\_versions}{$L\_t\_id \downarrow,\currs \downarrow$} \label{lin:checkVersion1}
\cmnts{From $\currs.vls$, identify the correct $version\_tuple$ means identfy the tuple which is having higher time-stamp but less then it} \label{lin:checkVersion2}
\State $\find(L\_t\_id \downarrow, \currs \downarrow, closest\_tuple \uparrow)$;\label{lin:checkVersion3}	
\cmnts{Got the closest\_tuple as $\langle j,val,mark,rvl,vnext \rangle$}\label{lin:checkVersion4}
%\ForAll {$v\_tuples \langle j,v,rl \rangle $ in $x \cdot vl$}
\ForAll {$T_k$ in $rvl$ of $closest\_tuple.j$}\label{lin:checkVersion5}
\cmnts{$T_k$ has already read the version created by $T_j$}\label{lin:checkVersion6}
\If {$(L\_t\_id < k)$}   \label{lin:checkVersion7}
\cmnts{If in $rvl$ of $closest\_tuple.j$, any higher time-stamp exists then $L\_t\_id$ then return $FALSE$}\label{lin:checkVersion8}
\State return $\langle FALSE\rangle$;  \label{lin:checkVersion9}
\EndIf\label{lin:checkVersion10}
\EndFor\label{lin:checkVersion11}
%\EndFor;
\cmnts{If in $rvl$ of $closest\_tuple.j$, there is no higher time-stamp exists then $L\_t\_id$ then return $TRUE$}\label{lin:checkVersion12}
\State return $\langle TRUE\rangle$;\label{lin:checkVersion13}
\EndProcedure\label{lin:checkVersion14}
\end{algorithmic}
%\end{multicols}
\end{algorithm}

\begin{figure}[tbph]
	\captionsetup{justification=centering}
	%\includegraphics[scale=0.7]{figs/ex1.pdf_t}
	%\centerline{\scalebox{0.7}{\input{ex1.pstex_t}}}
	\centerline{\scalebox{0.47}{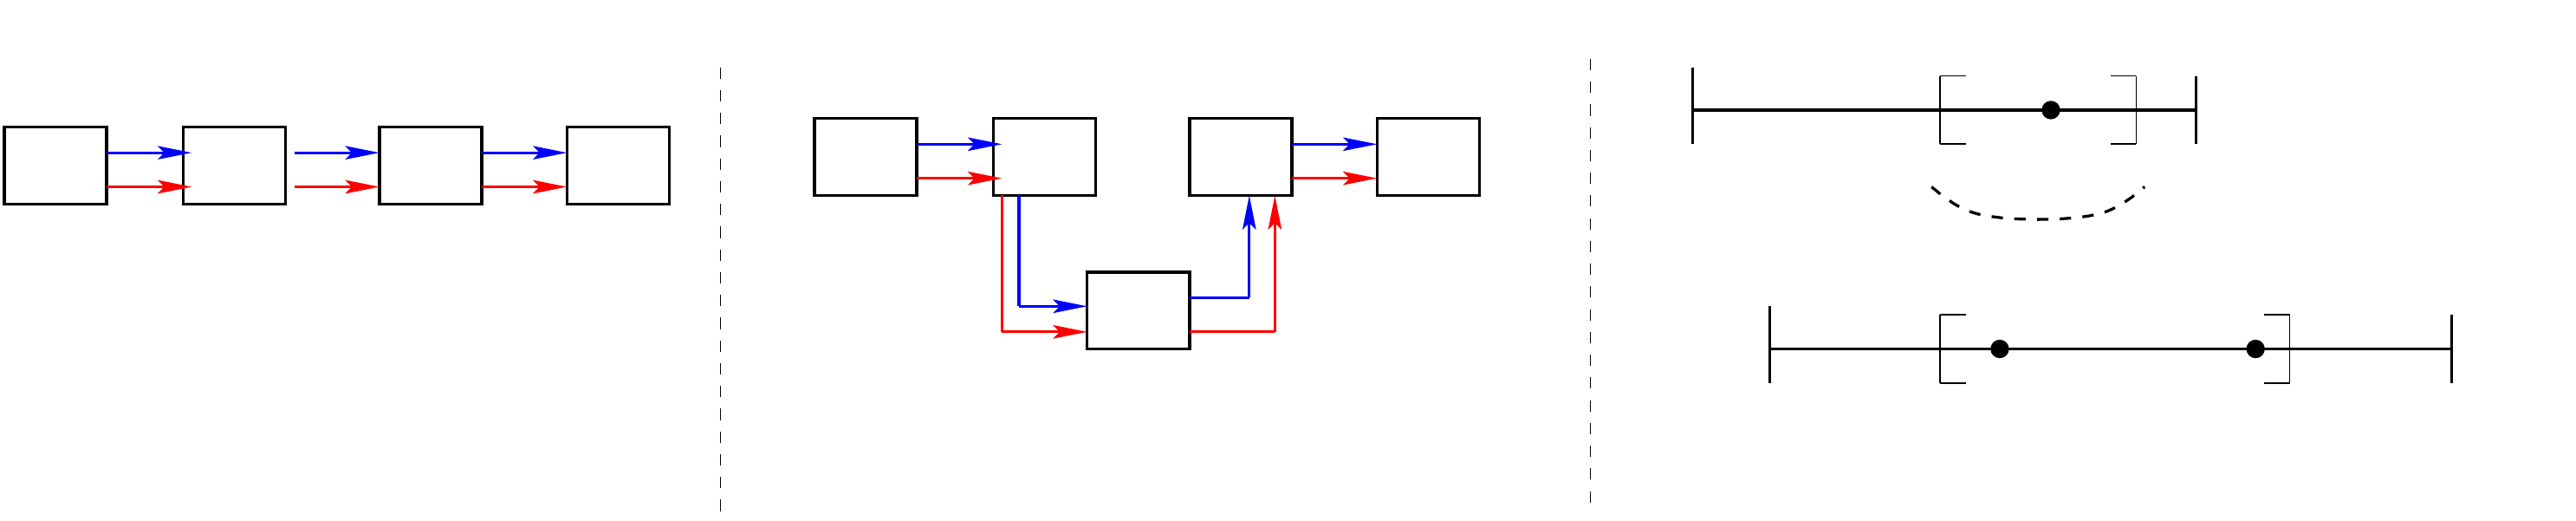}}
	\caption{Method validation}
	\label{fig:mvostm9}
\end{figure}
\cmnt{
\begin{figure}[tbph]
	%\includegraphics[scale=0.7]{figs/ex1.pdf_t}
	%\centerline{\scalebox{0.7}{\input{ex1.pstex_t}}}
	\centerline{\scalebox{0.5}{\input{figs/mvostm9.pdf_t}}}
	\caption{Method validation}
	\label{fig:mvostm9}
\end{figure}
}

%%%%%%%%%%%%%%%%%%%%%%%%%%%%%%%%%%%%%%%%%%%%%%%%%%%%%%%%%%%%%%%%%%%%%%%%%%
%---------------------------------methodValidation -------------------
%%%%%%%%%%%%%%%%%%%%%%%%%%%%%%%%%%%%%%%%%%%%%%%%%%%%%%%%%%%%%%%%%%%%%%%%%%

\begin{algorithm}[H]
\scriptsize
	\caption{\tabspace[0.2cm] methodValidation() : This method is called by the \rvmt{} and \upmt{}. It will identify the conflicts among the concurrent methods of different transactions at \Lineref{iv2}. It will be more clear by the \figref{mvostm9}, where two concurrent conflicting methods of different transactions are working on the same key $k_3$. Initially, at stage $s_1$ in \figref{mvostm9}.c) both the conflicting method optimistically (without acquiring locks) identify the same $\preds$ and $\currs$ for key $k_3$ from underlying DS in \figref{mvostm9}.a). At stage $s_2$ in \figref{mvostm9}.c), method $ins_1(k_3)$ of transaction $T_1$ acquired the lock on $\preds$ and $\currs$ and inserted the node into it (\figref{mvostm9}.b)). After successful insertion by $T_1$, $\preds$ and $\currs$ will change for $lu_2(k_3)$ at stage $s_3$ in \figref{mvostm9}.c). It will caught via method validation function at \Lineref{iv2} when $(\preds.\bn \neq G\_curr)$ for $lu_2(k_3)$. After that again it will find the new $\preds$ and $\currs$ for $lu_2(k_3)$ with the help of \nplsls{} method and eventually it will commit.}
		%\emph{DESCP}\tabspace: method validation for conflicting concurrent operations.\\
		%\emph{IN}\tabspace \tabspace[0.72cm]: $preds[]$, $currs[]$\\
		%\emph{OUT}\tabspace \tabspace[0.37cm]: $RETRY$, $OK$     }
	\label{algo:interferenceValidation}
			\setlength{\multicolsep}{0pt}
%	\begin{multicols}{2}
	\begin{algorithmic}[1]
\makeatletter\setcounter{ALG@line}{370}\makeatother	
		\Procedure{methodValidation}{$\preds \downarrow, \currs \downarrow, L\_op\_status \uparrow$} \label{lin:iv1}
	    \cmnts{Validating $\preds$ and $\currs$}
		\If{$((\bp.marked) || (\bc.marked) ||(\bp.\bn) \neq \bc || (\rp.\rn) \neq {\rc})$}  \label{lin:iv2}
		\cmnts{If validation fail then $L\_op\_status$ set as $RETRY$}
        \State $L\_op\_status$ $\gets$ RETRY

		\Else \label{lin:iv4}
		
	    \State $L\_op\_status$ $\gets$ OK

		\EndIf \label{lin:iv6}
				\State return $\langle L\_op\_status\rangle$ \label{lin:iv5};
	
		\EndProcedure \label{lin:iv7}
	\end{algorithmic}
%\end{multicols}
\end{algorithm}

%%%%%%%%%%%%%%%%%%%%%%%%%%%%%%%%%%%%%%%%%%%%%%%%%%%%%%%%%%%%%%%%%%%%%%%%%%
%------------------- find -----------------------
%%%%%%%%%%%%%%%%%%%%%%%%%%%%%%%%%%%%%%%%%%%%%%%%%%%%%%%%%%%%%%%%%%%%%%%%%%

\begin{algorithm}[H]
\scriptsize
	\caption{\tabspace[0.2cm] $L\_find()$ : This method is called by \npins{}, \rvmt{} and \upmt{}. It will check whether any method corresponding to $\left\langle L\_obj\_id, L\_key  \right\rangle$ is present in local log from \Lineref{findll4} to \Lineref{findll8}.}
		%\emph{DESCP}\tabspace: Checks weather any operation corresponding to $\left\langle obj\_id, key  \right\rangle$ is present in ll\_list.\\
		%\emph{IN}\tabspace \tabspace[0.72cm]: $\left\langle obj\_id, key  \right\rangle$  \\
		%\emph{OUT}\tabspace \tabspace[0.37cm]: $true, false$     }
	\label{algo:findInLL}
				\setlength{\multicolsep}{0pt}
%	\begin{multicols}{2}
	\begin{algorithmic}[1]
\makeatletter\setcounter{ALG@line}{380}\makeatother		
		\Procedure{L\_find}{$L\_t\_id \downarrow, L\_obj\_id \downarrow, L\_key \downarrow, L\_rec \uparrow$} \label{lin:findll1}
		
		%\State    /*get the tx id*/
		%\State $L\_t\_id$ $\gets$ getTS($t_i$) \label{lin:findll2};
		
		\State $L\_list$ $\gets$ \txgllist{} \label{lin:findll3}; 
	\cmnts{Every method first identify the node corresponding to the key into local log}
		\While{$(L\_rec_{i} \gets next(L\_list))$} \label{lin:findll4}
		\cmnts{Taking one by one $L\_obj\_id$ and $L\_key$ form $L\_rec$}
		\If{$((L\_rec_{i}.first = L\_obj\_id) \& (L\_rec_{i}.sec = L\_key))$} \label{lin:findll5}

		\State return $\langle TRUE, L\_rec \rangle$ \label{lin:findll6};
		\EndIf \label{lin:findll7}
		\EndWhile \label{lin:findll8}
		\State return $\langle FALSE, NULL \rangle$ \label{lin:findll9};
		\EndProcedure \label{lin:findll10}
	\end{algorithmic}
%	\end{multicols}
\end{algorithm}

%%%%%%%%%%%%%%%%%%%%%%%%%%%%%%%%%%%%%%%%%%%%%%%%%%%%%%%%%%%%%%%%%%%%%%%%%%
%------------------- releaseorderedlocks -----------------------
%%%%%%%%%%%%%%%%%%%%%%%%%%%%%%%%%%%%%%%%%%%%%%%%%%%%%%%%%%%%%%%%%%%%%%%%%%

\begin{algorithm}[H]
\scriptsize
	\caption{\tabspace[0.2cm] releaseOrderedLocks(): Release all locks in increasing order of their keys from \Lineref{rlock2} to \Lineref{rlock7}.}
		%\emph{DESCP}\tabspace: releases all locks taken during tryCommit\\
		%\emph{IN}\tabspace \tabspace[0.72cm]: $ordered\_ll\_list$\\
		%\emph{OUT}\tabspace \tabspace[0.37cm]:    }
	\label{algo:releaseorderedlocks}
			\setlength{\multicolsep}{0pt}
%	\begin{multicols}{2}
	\begin{algorithmic}[1]
	\makeatletter\setcounter{ALG@line}{391}\makeatother
		\Procedure{releaseOrderedLocks}{$L\_list \downarrow$} \label{lin:rlock1}
	\State    /*Releasing all the locks in increasing order of the keys */
		\While{($\textbf{$L\_rec_{i} \gets next(L\_list$})$)} \label{lin:rlock2}
		
		\State $L\_rec_{i}$.$\preds$.$\texttt{unlock()}$ \label{lin:rlock3};//$\Phi_{lp}$ 
		\State $L\_rec_{i}$.$\currs$.$\texttt{unlock()}$ \label{lin:rlock4};
		
		%\State $ll\_entry_i$.\textcolor{red}{$currs[0]$}.$\texttt{unlock()}$ \label{lin:rlock5};
		%\State $ll\_entry_i$.\textcolor{blue}{$currs[1]$}.$\texttt{unlock()}$ \label{lin:rlock6}; 
		\EndWhile \label{lin:rlock7}
		\State return $\langle void \rangle$;
		\EndProcedure \label{lin:rlock8}
	\end{algorithmic}
			
%	\end{multicols}
\end{algorithm}
%\end{multicols}

\begin{figure} [H]
	\captionsetup{justification=centering}
	%\centering
	%\includegraphics[scale=.5]{figs/fig3.png}
	%\includegraphics[scale=.5]{figs/fig3.pdf_t}
	\centerline{\scalebox{0.45}{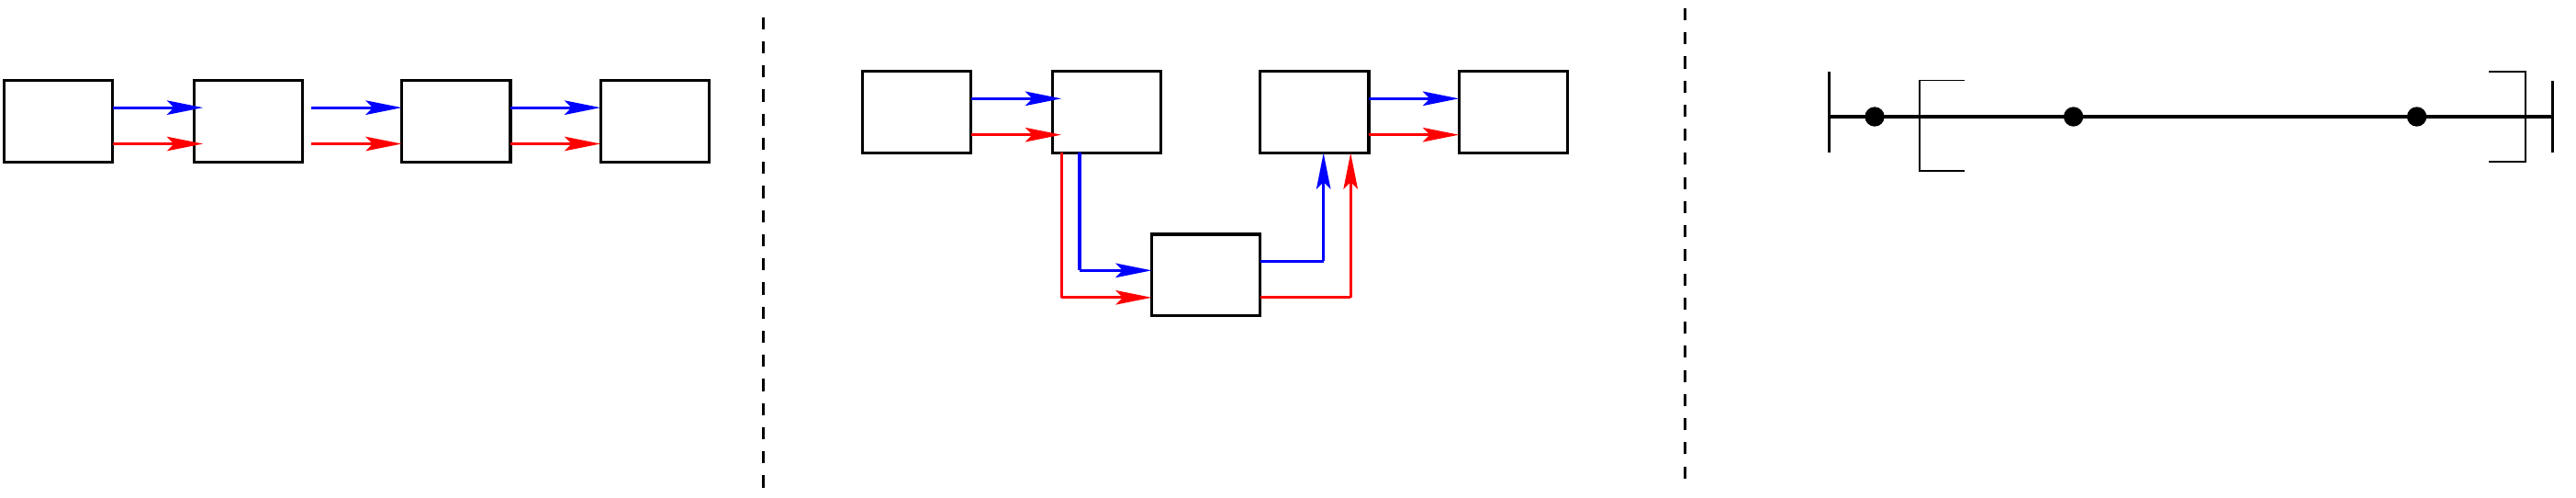}}
	\caption{Intra transaction validation}
	\label{fig:mvostmm11}
\end{figure}

\cmnt{
\begin{figure} [H]
	%\centering
	%\includegraphics[scale=.5]{figs/fig3.png}
	%\includegraphics[scale=.5]{figs/fig3.pdf_t}
	\centerline{\scalebox{0.5}{\input{figs/mvostm11.pdf_t}}}
	\caption{Intra transaction validation}
	\label{fig:mvostm11}
\end{figure}
}
%%%%%%%%%%%%%%%%%%%%%%%%%%%%%%%%%%%%%%%%%%%%%%%%%%%%%%%%%%%%%%%%%%%%%%%%%%
%%%%%%%%%%%%%%%%%%%%%%%%%%%%%%%%%intraTransValidation%%%%%%%%%%%%%%%%%%%%%%%%
%%%%%%%%%%%%%%%%%%%%%%%%%%%%%%%%%%%%%%%%%%%%%%%%%%%%%%%%%%%%%%%%%%%%%%%%%%

\begin{algorithm}[H]
\scriptsize
	\caption{\tabspace[0.2cm] intraTransValidation() : This method is called by \nptc{} only. If two $\upmt{s}$ within same transaction have at least one shared node among its recorded $\preds$ and $\currs$, in this case the previous $\upmt{}$ effect might be overwritten if the next $\upmt{}$ $\preds$ and $\currs$ are not updated according to the updates done by the previous $\upmt{}$. Thus to solve this we have intraTransValidation() after each $\upmt{}$ in $\nptc$. This will be more clear by the \figref{mvostmm11}, where two \upmt{s} of same transaction $T_1$ are $ins_{11}(k_3)$ and $ins_{12}(k_5)$ (\figref{mvostmm11}.c)). At stage $s_1$ in \figref{mvostmm11}.c) both the \upmt{s} identify the same $\preds$ and $\currs$ from underlying DS (\figref{mvostmm11}.a)). After the successful insertion done by first \upmt{} at stage $s_2$ in \figref{mvostmm11}.c), key $k_3$ is part of underlying DS (\figref{mvostmm11}.b)). At stage $s_3$ in \figref{mvostmm11}.c) if we will not update the $\preds$ and $\currs$ for $ins_{12}(k_5)$ then it will overwrite the previous method updates. To resolve this issue we are doing the intraTransValidation() after each \upmt{} to assign the appropriate $\preds$ and $\currs$ for the upcoming \upmt{} of same transaction.}
		%\emph{DESCP}\tabspace: program order validation\\
		%\emph{IN}\tabspace \tabspace[0.72cm]: $ll\_entry_i$  \\
		%\emph{OUT}\tabspace \tabspace[0.37cm]: $preds[], currs[]$}
	\label{algo:povalidation}
	\setlength{\multicolsep}{0pt}
%		\begin{multicols}{2}
	\begin{algorithmic}[1]
\makeatletter\setcounter{ALG@line}{399}\makeatother		
		\Procedure{intraTransValidation}{$L\_rec_{i} \downarrow, \preds \uparrow, \currs \uparrow$} \label{lin:threadv1}

	\State $L\_rec.getAllPreds\&Currs(L\_rec$ $\downarrow$, $\preds$ $\uparrow$, $\currs$ $\uparrow$) \label{lin:threadv2};	
				%\State \llgallpc{} \label{lin:threadv2};
				\cmnts{if $\bp$ is marked or $\bc$ is not reachable from $\bp.\bn$ then modify the next consecutive \upmt{} $\bp$ based on previous \upmt{}}
				\If{$(($$\bp$.\textup{marked}$) ||$ $($ $\bp$.\textup{\bn}$)$ != $\bc$$))$} \label{lin:threadv3}
				\cmnts{find $k$ < $i$; such that $le_k$ contains previous update method on same bucket }
				\If{$(($$L\_rec_{k}$.\textup{opn}$)$ $=$ INSERT$)$} \label{lin:threadv4}
				
				\State $L\_rec_{i}$.$\bp$.$\texttt{unlock()}$ \label{lin:thredv4-5};
				\State $\bp$ $\gets$ ($L\_rec_{k}.\bp.\bn)$ \label{lin:threadv5};
				\State $L\_rec_{i}$.$\bp$.$\texttt{lock()}$ \label{lin:thredv5-5};		
				\Else \label{lin:threadv6}
				\cmnts{\upmt{} method $\bp$ will be previous method $\bp$}
				\State $L\_rec_{i}$.$\bp$.$\texttt{unlock()}$ \label{lin:thredv6-5};
				\State $\bp$ $\gets$ ($L\_rec_{k}$.$\bp$) \label{lin:threadv7};
				
				\State $L\_rec_{i}$.$\bp$.$\texttt{lock()}$ \label{lin:thredv7-5};
				\EndIf \label{lin:threadv8}
				
				\EndIf \label{lin:threadv9}
				\cmnts{if $\rc$ \& $\rp$ is modified by prev operation then update them also}
				\If{$($$\rp$.\textup{\rn} != $\rc$$)$} \label{lin:threadv10}
				\State $L\_rec_{i}$.$\rp$.$\texttt{unlock()}$
				\State $\rp$ $\gets$ ($L\_rec_{k}$.$\rp.\rn$)  \label{lin:threadv11}; 
				\State $L\_rec_{i}$.$\rp$.$\texttt{lock()}$
				\EndIf \label{lin:threadv12}
				\State return $\langle \preds, \currs\rangle$;
	\cmnt{

	        \State $L\_rec.getAllPreds\&Currs(L\_rec_{i}$ $\downarrow$, $G\_pred$ $\uparrow$, $G\_curr$ $\uparrow$) \label{lin:threadv2};	
		%\State \llgallpc{} \label{lin:threadv2};
	%\State    /*if $\bp$ is marked or $\bc$ is not reachable from $\bp.\bn$ then modify the next consecutive \upmt{} $\bp$ based on previous \upmt{}*/
		\If{$(G\_pred.knext \neq G\_curr)$} \label{lin:threadv3}
		\State    /*Find $k$ $>$ $i$; such that $L\_rec_{k}$ contains next update method on same bucket */
		\If{$((($$L\_rec_{k}$.\textup{L\_opn}$)$ $=$ INSERT$)$ $||$ $(($$L\_rec_{k}$.\textup{L\_opn}$)$ $=$ DELETE$))$} \label{lin:threadv4}
		
	\State $L\_rec_{k}$.$G\_pred$.$\texttt{unlock()}$ \label{lin:thredv4-5};
		\State $G\_pred$ $\gets$ ($L\_rec_{i}.G\_pred.knext)$ \label{lin:threadv5};
	\State $L\_rec_{k}$.$G\_pred$.$\texttt{lock()}$ \label{lin:thredv5-5};		
		%\Else \label{lin:threadv6}
	%\State    /*\upmt{} method $\bp$ will be previous method $\bp$*/
	%\State $L\_rec_{i}$.$G\_pred$.$\texttt{unlock()}$ \label{lin:thredv6-5};
	%	\State $G\_pred$ $\gets$ ($L\_rec_{i}$.$G\_pred$) \label{lin:threadv7};
		
	%		\State $L\_rec_{i}$.$G\_pred$.$\texttt{lock()}$ \label{lin:thredv7-5};
		\EndIf \label{lin:threadv8}
		
		\EndIf \label{lin:threadv9}
	\State return $\langle G\_pred, G\_curr\rangle$;
	}
	\EndProcedure	
	\end{algorithmic}
%		\end{multicols}
\end{algorithm}

%%%%%%%%%%%%%%%%%%%%%%%%%%%%%%%%%%%%%%

%%%%%%%%%%%%%%%%% Garbage Collection 

%%%%%%%%%%%%%%%%%%%%%%%%%%%%%%%%%%%%%%%%%%%%%%%%%

\section{Garbage Collection}
\label{sec:gc}
We have performed garbage collection method to delete the unwanted version of keys i.e. if the particular version corresponding to any key is not going to use in future then we can delete that version. For the better understanding of it please consider \figref{mvostm4}. Here, we are having 3 versions of key $k_1$ with timestamp 0, 15 and 25 respectively. Each version is having 5 fields described in \secref{mvdesign}. Now, consider the version 15, there exist the next version 25 and all the transactions between 15 to 25 has been terminated (either commit or abort) then we are deleting version 15. Similarly, we can delete other versions corresponding to each key as well and optimize the memory. 

\begin{figure} [H]
	%\centering
	%\includegraphics[scale=.5]{figs/fig3.png}
	%\includegraphics[scale=.5]{figs/fig3.pdf_t}
	\centerline{\scalebox{0.35}{\input{figs/mvostm4.pdf_t}}}
	\caption{Data Structures for Garbage Collection}
	\label{fig:mvostm4}
\end{figure}

\begin{algorithm}[H] 
\scriptsize
\label{alg:begin1} 
\caption{STM $begin()$: Invoked by a thread to being a new transaction $T_i$}
	\setlength{\multicolsep}{0pt}
	%	\begin{multicols}{2}
\begin{algorithmic}[1]
%\State lock $\tcntr$;
\makeatletter\setcounter{ALG@line}{423}\makeatother
\Procedure{STM begin}{$L\_t\_id \uparrow$}
\State /*Creating a local log for each transaction*/
\State \txll $\gets$ create new \txllf;  
%\State /*Acquiring lock on live set of transaction*/
%\State $\livetx.lock()$;  
\State /*Get $t\_id$ from $\cnt$*/
\State \txll.$L\_t\_id$ $\gets$ $\cnt$;  
\State /*Incremented $\cnt$*/
\State $\cnt$ $\gets$ \gi;  
%\State add $t\_id$ to $\livetx$; 
%\State /*Release lock on live set of transaction*/
%\State $\livetx.unlock()$;
\State $\livel.lock()$; \label{lin:beginit}
\State add $L\_t\_id$ to $\livel$; 
\State $\livel.unlock()$;
\State return $\langle L\_t\_id \rangle$; 
\EndProcedure
%\State unlock $\tcntr$;
%\State return $i$; \label{lin:begfin}
%\EndFunction{$\begtrans${}}
\end{algorithmic}
%\end{multicols}
\end{algorithm}

\begin{algorithm}[H]  
\scriptsize
\label{alg:instuple}
\caption{$\instup()$: Inserts the version tuple for $(L\_t\_id,v)$ created by the transaction $T_i$ into the version list of $L\_key$}
	\setlength{\multicolsep}{0pt}
%		\begin{multicols}{2}
\begin{algorithmic}[1]
\makeatletter\setcounter{ALG@line}{435}\makeatother
\Procedure{ins\_tuple}{$L\_key \downarrow, L\_t\_id\downarrow, v\downarrow, NULL\downarrow, NULL\downarrow$}
\State /*Initialize $cur\_tuple$*/
\State $cur\_tuple = \langle L\_t\_id, val, F, NULL, NULL \rangle$; 
\State /* Finds the tuple with the largest timestamp smaller than i */
\State $\find(L\_t\_id \downarrow, L\_key \downarrow, prev\_tuple \uparrow)$; \label{lin:prevtup}
\State /*$prev\_tuple$ is $\langle ts, val, mark, rvl, nts\rangle$*/
\State $cur\_tuple.nts = prev\_tuple.nts$;
\State $prev\_tuple.nts = L\_t\_id$;
\State insert $cur\_tuple$ into $L\_key.vl$ in the increasing order of timestamps;  
\State /* $\lvert L\_key.vl \lvert$ denotes number of versions of $L\_key$ created and threshold is a predefined value. */
\If {($\lvert L\_key.vl \lvert > threshold$)} 
\State /*If number of created versions for $L\_key$ crossed the threshold value then calling the Garbage Collection*/ 
\State $gc(L\_key)$;
\EndIf 
\State return $\langle void \rangle$
\EndProcedure
\end{algorithmic}
%\end{multicols}
\end{algorithm}

\begin{algorithm}[H]
\scriptsize
\caption{STM $\gc()$: Unused version of a \tobj{} $L\_key$ will deleted from $L\_key.vl$}
	\setlength{\multicolsep}{0pt}
%		\begin{multicols}{2}
\begin{algorithmic}[1]
\makeatletter\setcounter{ALG@line}{451}\makeatother
\Procedure{gc}{$L\_key \downarrow$}
\State $\livel.lock()$;
\State /*\tobj{} $L\_key$ is already locked*/
\ForAll {$(cur\_tuple \in L\_key.vl)$} 
\If {$(cur\_tuple.nts == NULL)$}
\State /* If $nts$ is NULL, check the next tuple in the version list */
\State continue; 
\EndIf
\State $j = cur\_tuple.ts + 1$;
\State /*Check for all ids $j$ in the range $j < nts$*/
\While {$(j < cur\_tuple.nts)$} 
\If {$(j \in \livel)$}
\State /* If any tuples with timestamp $j$, such that  $i< j < nts$ have not terminated (means exist in $liveList$) then $cur\_tuple$ can't be deleted*/

\State break;
\EndIf
\EndWhile
\State /* If all the tuples with timestamp $j$, such that  $i< j < nts$ have terminated then $cur\_tuple$ can be deleted*/
\State delete $cur\_tuple$;
\EndFor 
\State /* $\livel$ is not unlocked when this function returns */
%\State unlock $\livel$;
\State return $\langle void \rangle$
\EndProcedure
\end{algorithmic}
%\end{multicols}
\end{algorithm}
